# Supplementary material for: Wave propagation in micromorphic anisotropic continua with an application to tetragonal crystals
Source: arXiv:2009.09825 source file (2020-09-21)
Supplement: Supplementary file 1 [file appendix2a.tex]

\subsection{The eigenvector components}

\subsection{Subspace $\caU_{1}$}\label{eigencompU1}
The real coefficients $a, b, c, d, e$ and $f$ are given by (\ref{compoU1micro}): [a, b e c vanno con $-\omega$]
\begin{itemize}
\item $\Cb_{1}$
\begin{align}
\alpha_{1} &=\frac{1}{\Delta_{1}} (h(d(l^2+bf)+a(l^2-bc)+2 egl-bg^2+ e^2(c-f))\nonumber\\
& +g(a(-l^2-bf)+d(bc-l^2)+ e^2(f-c))\nonumber\\
&-3 eh^2l+ eg^2l + ea(f+c)l+ ed(-f-c)l+bh^3)\nonumber\\ 
\beta_{1} &=\frac{1}{\Delta_{1}} -(h(a(l^2+bf)+d(l^2-bc)-2 egl+ e^2(c-f))\nonumber\\
& +g(d(-l^2-bf)+a(bc-l^2)+ e^2(f-c))+h^2(bg- el)\nonumber\\
&+3 eg^2l + ed(f+c)l+ ea(-f-c)l-bg^3)\nonumber\\ 
\gamma_{1} &=\frac{1}{\Delta_{1}} -(h(2gl(d+a)- eg^2+ e(d-a)(f+c))\nonumber\\
& +h^2(-l(a+d)- eg)-g^2l(a+d)+(a^2-d^2)(f+c)l+ e(h^3 + g^3)+eg(d-a)(f+c)) \nonumber\\ 
\delta_{1} &=\frac{1}{\Delta_{1}} -((d^2-a^2)(l^2+bf) +2h(el(a-d)+(e^2-ab)g)\nonumber\\
& +2gel(a-d)+(bd- e^2)(h^2 +g^2)-2 e^2f(a+d)) \nonumber\\
\epsilon_{1}&=1\nonumber
\end{align}
where
\begin{equation*}
\Delta_{1}=(a^2-d^2)(l^2-bc)+2(el(h+g)- e^2c)(d-a)+2(e^2-bd)gh +(ab- e^2)(h^2+g^2)\,.
\end{equation*}
\item $\Cb_{2}$
\begin{align}
\Delta_{2}=\Delta_{1}\,,
\end{align}
\begin{align}
\alpha_{2}&=-\beta_{1}\nonumber\\ 
\beta_{2}&=-\alpha_{1}\nonumber\\ 
\gamma_{2}&=-\gamma_{1}\nonumber\\ 
\delta&=1\nonumber\\
\epsilon_{2} &=\delta_{1}\nonumber
\end{align}
\item $\Cb_{3}$
\begin{align}
\Delta_{3}=(h^4+(-2g^2+2df-2ac)h^2+(4cd-4af)gh+g^4 +(2df-2ac)g^2+d^2(f^2-c^2)-a^2f^2+a^2c^2)\,,
\end{align}
\begin{align}
\alpha&=\frac{ -(h(d(fl+cl)-g^2l-afl-acl+c(2 e-2f)g) +g(d(fl+cl)-afl-acl)+h^2(-gl+ ef-c^2)+h^3l+g^3l +( ef-c^2)g^2+d( ef^2- ec^2)-acf^2+ac^3) }{\Delta}\nonumber\\ 
\beta&=\frac{ -(h(d(fl+cl)-g^2l-afl-acl+(2c^2-2 ef)g) +g(d(fl+cl)-afl-acl)+h^2(c(f- e)-gl)+h^3l+g^3l +c(f- e)g^2+d(cf^2-c^3)- eaf^2+ eac^2) }{\Delta}\nonumber\\ 
\gamma&=1\nonumber\\
\delta&=\frac{ -(h(g(2dl+2al)- eg^2+d( ef+c^2)+ac(-f- e)) +d^2(-fl-cl)+h^2(-dl-al-cg)+g^2(-dl-al)+a^2fl+a^2cl + eh^3+cg^3+(cd(f+ e)- eaf-ac^2)g) }{\Delta}\nonumber\\ 
\epsilon&=\frac{ (h(g(2dl+2al)-cg^2+cd(f+ e)- eaf-ac^2) +d^2(-fl-cl)+h^2(-dl-al- eg)+g^2(-dl-al)+a^2fl+a^2cl +ch^3+ eg^3+(d( ef+c^2)+ac(-f- e))g) }{\Delta}\nonumber
\end{align}
\item $\Cb_{4}$
\begin{align}
\Delta_{4}=(a((-2f-2c)l^2+b(c^2-f^2))+h^2(l^2-bc)+g^2(l^2-bc) +h(g(-2l^2-2bf)+ e(2f+2c)l) + e(2f+2c)gl+ e^2(f^2-c^2))\,,
\end{align}
\begin{align}
\alpha &=\frac{ (d((2f+2c)l^2+b(f^2-c^2))+h^2(l^2+bf)+g^2(l^2+bf) +h(g(2bc-2l^2)+ e(-2f-2c)l) + e(-2f-2c)gl+ e^2(c^2-f^2)) }{\Delta}\nonumber\\ 
\beta&=1\nonumber\\
\gamma &=\frac{ -(h(-g^2l+d(f+c)l+a(-f-c)l+ e(2c-2f)g) +h^2( e(f-c)-gl)+g(d(f+c)l+a(-f-c)l)+h^3l+g^3l + e(f-c)g^2+ ed(f^2-c^2)+ ea(c^2-f^2)) }{\Delta}\nonumber\\ 
\delta &=\frac{ (h(d(l^2+bf)+a(l^2-bc)+2 egl-bg^2+ e^2(c-f)) +g(a(-l^2-bf)+d(bc-l^2)+ e^2(f-c))-3 eh^2l+ eg^2l + ea(f+c)l+ ed(-f-c)l+bh^3) }{\Delta}\nonumber\\ 
\epsilon &=\frac{ (h(a(l^2+bf)+d(l^2-bc)-2 egl+ e^2(c-f)) +g(d(-l^2-bf)+a(bc-l^2)+ e^2(f-c))+h^2(bg- el)+3 eg^2l + ed(f+c)l+ ea(-f-c)l-bg^3) }{\Delta}\nonumber
\end{align}
\item $\Cb_{5}$
\begin{align}
\Delta_{5}=(a((-2f-c)l^2+ e(bc-l^2)-bf^2) +h^2(l^2-bc)+g^2(l^2- eb)+h(g(-2l^2-2bf)+ e(2f+2c)l) +g(2 efl+2 e^2l)+ e^2f^2- e^3c)
\end{align}
\begin{align}
\alpha&=1\nonumber\\
\beta &=\frac{ (d( e(l^2-bc)+(2f+c)l^2+bf^2) +h^2(l^2+bf)+g^2(l^2+bf) +h(g(-2l^2+bc+ eb)+ e(-2f-c)l- e^2l) +g( e(-2f-c)l- e^2l)- e^2f^2+ e^3c) }{\Delta}\nonumber\\ 
\gamma &=\frac{ -(g(d(fl+ el)+a(-f-c)l) +h(a(-fl- el)-g^2l+d(f+c)l+( e(c-2f)+ e^2)g) +h^2( e(f-c)-gl)+h^3l+g^3l+( ef- e^2)g^2+d( ef^2- e^2c) +a( e^2c- ef^2)) }{\Delta}\nonumber\\ 
\delta &=\frac{ -(h(a(l^2+bf)+d(l^2-bc)-2 egl+ e^2(c-f)) +g(d(-l^2-bf)+a(bc-l^2)+ e^2(f-c))+h^2(bg- el)+3 eg^2l + ed(f+c)l+ ea(-f-c)l-bg^3) }{\Delta}\nonumber\\ 
\epsilon&=\frac{ -(h(d(l^2+bf)+a(l^2- eb)+2 egl-bg^2- e^2f+ e^3) +g(a(-l^2-bf)+d( eb-l^2)+ e^2f- e^3)+a( efl+ e^2l) +d(- efl- e^2l)-3 eh^2l+ eg^2l+bh^3) }{\Delta}\nonumber
\end{align}
\end{itemize}

%\begin{align}
%\alpha_{1}&=\frac{(b-\omega_{1}^{2})(c-f-\omega_{1}^{2})}{(b-\omega_{1}^{2})(g+h)-2el}\,,\quad\gamma_{1}=\frac{-2e(c-f-\omega_{1}^{2})}{(b-\omega_{1}^{2})(g+h)-2el}\,,\\
%\alpha_{2}&=\frac{2l^{2}-(b-\omega_{2}^{2})(c-f-\omega_{2}^{2})}{(b-\omega_{2}^{2})(g+h)-2el}\,,\quad\gamma_{2}=\frac{2e(c-f-\omega_{2}^{2})-2l(g+h)}{(b-\omega_{2}^{2})(g+h)-2el}\,,\nonumber\\
%\alpha_{3}&=\frac{l(g+h)-e(c-f-\omega_{3}^{2})}{(a+d-\omega_{3}^{2})(c-f-\omega_{3}^{2})-(g+h)^2}\,,\delta_{3}=\frac{e(g+h)-l(a+d-\omega_{3}^{2})}{(a+d-\omega_{3}^{2})(c-f-\omega_{3}^{2})-(g+h)^2}\,,\nonumber\\
%\gamma_{4}&=\frac{(\omega_{4}^{2}-a-d)(g+l)+2e(g+h)}{(b-\omega_{4}^{2})(g+h)+e(g+l)}\,,\quad\delta_{4}=-\frac{2e^{2}+(b-\omega_{4}^{2})(\omega_{4}^{2}-a-d)}{(b-\omega_{4}^{2})(g+h)+e(g+l)}\,,\nonumber\\
%\gamma_{5}&=-\frac{2l(\omega_{5}^{2}-a-d)+2e(g+h)}{(b-\omega_{5}^{2})(g+h)-2el}\,,\quad\delta_{5}=\frac{(b-\omega_{5}^{2})(\omega_{5}^{2}-a-d)+2e^2}{(b-\omega_{5}^{2})(g+h)-2el}\,.\nonumber
%\end{align}

\subsubsection{Subspace $\caN_{1}$}

The complex coefficients $a, b, c, f, g, h$ and $l$ are given by (\ref{definLS1}):
\begin{align}\label{eigencompN1}
&\beta_{2}=\frac{c^{*}l-b^{*}(g-\omega_{2}^{2})}{(f+h-\omega_{2}^{2})(g-\omega_{2}^{2})+2l^{2}}\,,&\gamma_{2}=\frac{2b^{*}l-c^{*}(f+h-\omega_{2}^{2})}{(f+h-\omega_{2}^{2})(g-\omega_{2}^{2})+2l^{2}}\,,\nonumber\\
&\alpha_{3}=\frac{c(\omega_{3}^{2}-f-h)-2bl}{(a-\omega_{3}^{2})(f+h-\omega_{3}^{2})+2bb^{*}}\,,&\beta_{3}=\frac{(\omega_{3}^{2}-a)l-cb^{*}}{(a-\omega_{3}^{2})(f+h-\omega_{3}^{2})+2bb^{*}}\,,\nonumber\\
&\alpha_{4}=\frac{2((g-\omega_{4}^{2})^{2}b-lc^{*})}{(a-\omega_{4}^{2})(g-\omega_{4}^{2})-cc^{*}}\,,&\gamma_{4}=\frac{2(l(a-\omega_{4}^{2})-bc^{*})}{(a-\omega_{4}^{2})(g-\omega_{4}^{2})-cc^{*}}\,,\nonumber
\end{align}

\subsubsection{Subspace $\caN_{3}$}\label{eigencompN3}

Ricordarsi che $c$ e $d$ vanno messi complessi coniugati e che bisogna sostituire ad $a$ $a-\omega^{2}$ ecc.
\begin{itemize}
\item
$w_{1}=\{\alpha_{1}\,,\beta_{1}\,,\gamma_{1}\,,\delta_{1}\,,\epsilon_{1}\,,1\}$
\begin{align}
\alpha_{1}&=-\frac{dg(a(g^2- ef)+3c^2f)+acf( ef-g^2) +cd^2(-2g^2- ef)+ ed^3g -c^3f^2 }{\Delta}\,,\nonumber\\ 
\beta_{1} &=\frac{b (d(g^3- efg)+c( ef^2-fg^2)) }{\Delta}\,,\nonumber\\ 
\gamma_{1} &=-\frac{b(d^2g^2-2cdfg+c^2f^2) }{\Delta}\,,\nonumber\\ 
\delta_{1} &=\frac{(a^2-b^2)(g^3- efg)-d(ac(3g^2- ef)+c^3f+d^2g(2c^2+ea)+ac^2fg+ ecd^3}{\Delta}\,,\nonumber\\ 
\epsilon_{1} &=\frac{ b(g(c^2f+ ed^2)-cd(g^2+ef)) }{\Delta}\,,\nonumber
\end{align}
where
\begin{align}
\Delta&=d^2(a(g^2-2 ef)+c^2f)+f(b^2-a^2)(g^2- ef)+2acdfg-2cd^3g-ac^2f^2 + ed^4\,.\nonumber
\end{align}
\item
$w_{2}=\{\alpha_{2}\,,\beta_{2}\,,\gamma_{2}\,,\delta_{2}\,,1\,,\theta_{2}\}$
\begin{align}
\alpha_{2} &=\frac{b(ed-cg)( ef-g^2)}{\Delta}\,,\nonumber\\ 
\beta_{2} &=\frac{a(cg-de)( ef-g^2)+dc^2(2g^2+ ef)-c^3fg -3 ecd^2g+ e^2d^3}{\Delta}\,,\nonumber\\ 
\gamma_{2} &=\frac{g(a^2-b^2)(g^2- ef)-d(ac(3g^2- ef)+c^3f)-d^2(-2c^2g- eag)+ac^2fg-ecd^3}{\Delta}\,,\nonumber\\ 
\delta_{2} &=-\frac{b(c^2g^2-2 ecdg+ e^2d^2) }{\Delta}\,,\nonumber\\ 
\theta_{2} &=\frac{ b(g(c^2f+ ed^2)-cd(g^2+ef)) }{\Delta}\,,\nonumber
\end{align}
where
\begin{align}
\Delta&=e(b^2-a^2)(g^2- ef)+ac^2(g^2-2 ef)+cdg(2 ea-2c^2)+c^4f +( c^2- ea)ed^2\,.\nonumber
\end{align}
\item
$w_{3}=\{\alpha_{3}\,,\beta_{3}\,,\gamma_{3}\,,1\,,\epsilon_{3}\,,\theta_{3}\}$
\begin{align}
\alpha_{3}&=\frac{ a(g^2-cf)+c^2(d-g)}{d(c^2-ag)-bc^2}\,,\nonumber\\ 
\beta_{3} &=\frac{ g(d^2-bg)+fc(b-d)}{d(c^2-ag)-bc^2}\,,\nonumber\\ 
\gamma_{3} &=\frac{e(g^2-cf)(b^2-a^2)+ac^2g(g+e)-d(ac^2- ebcf-c^4)-ac^3f-ebd^2g-c^4g}{(cg-ed)(d(ag-c^2)+bc^2)\,,}\nonumber\\ 
\epsilon_{3}&=\frac{ bcg+adf-cd^2}{d(c^2-ag)-bc^2}\,,\nonumber\\ 
\theta_{3} &=\frac{(g^3-cfg)(a^2-b^2)-dc(g(ag+bf)+c(cg-af-ag))-d^2(c^3-bg^2)-ac^2g^2}{(cg-ed)(d(ag-c^2)+bc^2)}\,.\nonumber
\end{align}

\item
$w_{4}=\{\alpha_{4}\,,\beta_{4}\,,1\,,\delta_{4}\,,\epsilon_{4}\,,\theta_{4}\}$
\begin{align}
\alpha_{4}&=\frac{b(dg-cf)(g^2- ef)}{\Delta}\,,\nonumber\\ 
\beta_{4}&=\frac{a(cf-dg)(g^2- ef)+cd^2(2g^2+ef)-3dgc^2f-d^3g+c^3f^2}{\Delta}\,,\nonumber\\
\delta_{4}&=\frac{ b(g(c^2f+ ed^2)-cd(g^2+ef)) }{\Delta}\,,\nonumber\\ 
\epsilon_{4}&=\frac{g(a^2-b^2)(g^2- ef)-d(ac(3g^2- ef)-c^3f)+gd^2(2c^2+ea)+ac^2fg-ecd^3}{\Delta}\,,\nonumber\\ 
\theta_{4}&=-\frac{b(dg-cf)^2 }{\Delta}\,,\nonumber
\end{align}
where
\begin{align}
\Delta&=d^2(a(g^2-2 ef)+c^2f)+f(a^2-b^2)( ef-g^2) +2cdg(af-d^2)-ac^2f^2 + ed^4\,.\nonumber
\end{align}
\item
$w_{5}=\{\alpha_{5}\,,1\,,\gamma_{5}\,,\delta_{5}\,,\epsilon_{5}\,,\theta_{5}\}$
\begin{align}
\alpha_{5} &=\frac{b(ef-g^2)}{a(g^2- ef)-2cdg+c^2f+ ed^2}\,,\nonumber\\
\gamma_{5}&=\frac{ cf-dg}{g^2- ef}\,, \nonumber\\
\delta_{5} &=\frac{ -b( ed-cg)}{a(g^2- ef)-2cdg+c^2f+ ed^2}\,, \nonumber\\
\epsilon_{5} &=\frac{ed-cg}{g^2- ef}\,, \nonumber\\
\theta_{5} &=\frac{ b(bg-cf)}{a(g^2- ef)-2cdg+c^2f+ ed^2}\,.\nonumber
\end{align}
\item
$w_{6}=\{1\,,\beta_{6}\,,\gamma_{6}\,,\delta_{6}\,,\epsilon_{6}\,,\theta_{6}\}$
\begin{align}
\beta_{6} &=\alpha_{5}\,,\quad\delta_{6}=\epsilon_{5}\,,\quad\epsilon_{6}=\delta_{5}\,,\quad\theta_{6}=\gamma_{5}\,,\\
\gamma_{6} &=\frac{ b(dg-cf)}{a(g^2- ef)-2cdg+c^2f+ ed^2}\,. \nonumber
\end{align}
\end{itemize}

\subsubsection{Subspace $\caM_{1}$}

\begin{itemize}
\item
$w_{1}=\{\alpha_{1}\,,\beta_{1}\,,\gamma_{1}\,,\delta_{1}\,,\epsilon_{1}\,,1\}$

All the components must be divided by:
\begin{align}
\Delta&=(((2h-2f)l^2-gh^2+f^2g)q^2 +(c((2f-2h)lp+l(fn-hn)+((f-h)l+2h^2-2f^2)m) +b((2gh-2fg)p+ghn-fgn+((4f-4h)l+gh-fg)m)) q +a((fg-l^2)p^2+(l^2n-ghn+(l^2+(2h-2f)l-gh)m)p +m(l(hn-fn)-l^2n+fgn)+((h-f)l-h^2+f^2)m^2 +(2df-2dh)l^2+dgh^2-df^2g) +bc (2lp^2+((-2l-2h+2f)m-2ln)p+m(2ln-hn+fn)+(f-h)m^2 +(4dh-4df)l) +b^2(-gp^2+(gn+gm)p-gmn+(2h-2f)m^2-2dgh+2dfg) +c^2(-fp^2+(hn+hm)p-fmn-dh^2+df^2))\,.\nonumber
\end{align}

\begin{align}
A&=2l^2-g(h+f)\nonumber\\
B&=\nonumber\\
C&=\nonumber\\
D&=\nonumber\\
E&=\nonumber\\
F&=\nonumber\\
G&=\nonumber\\
H&=\nonumber
\end{align}

\begin{align}
\alpha_{1}&=\frac{-1}{\Delta}((Ap^2+(-3l^2n+ghn+2fgn+(gh-l^2)m)p +l^2(n^2+(d+e)h-2(d+e)f) -ghn^2+m(l(hn-fn)+l^2n-fgn) +(f-h)lm^2+(-d- e)gh^2+(d+ e)f^2g) q +c(-lp^3+(ln+(h+f)m)p^2 +(m(ln-hn-2fn)-hm^2+((-d- e)h+(d+ e)f)l)p +m(hn^2+l(-n^2- eh+ ef)+(d+ e)h^2+(-d- e)f^2) +l(dfn-dhn)+fm^2n) +b(gp^3+(-gn-2lm)p^2 +(m(3ln-gn)+lm^2+(d+ e)gh+(-d- e)fg)p +m(gn^2+l(-n^2+(-2d-2 e)h+(2d+2 e)f)+ egh - efg)+m^2(-ln-hn+fn)+dghn-dfgn +(h-f)m^3)) \nonumber\\ 
\beta_{1}&=\frac{-1}{\Delta}((Ap-l^2n+ghn+(fg-l^2)m)q^2 +(c(-3lp^2+(ln+(l+2h+2f)m)p+m(ln-2hn)-2fm^2 +((-d- e)h+(d+ e)f)l) +b(3gp^2+((-4l-g)m-gn)p+m(2ln-gn)+2lm^2+(d+ e)gh +(-d- e)fg)) q +a(-gp^3+3lmp^2 +(m(gn-ln)+(-l-h-f)m^2+( e-d)l^2- egh+dfg)p +m^2(hn-ln)+dl^2n-dghn+fm^3 +(- el^2+((d+ e)h+(-d- e)f)l+ efg)m) +c^2(p^3+(-mn+ eh-df)p+dhn- efm) +bc (-3mp^2+(mn+m^2+(2d-2 e)l)p+m^2n-2dln +(2 el+(-d- e)h+(d+ e)f)m) +b^2((2m^2+( e-d)g)p-m^2n+dgn-m^3- egm)) \nonumber\\ 
\gamma_{1}&=\frac{1}{\Delta} ((Ap-l^2n+fgn+(gh-l^2)m)q^2 +(c(-lp^2+((2h+2f)m-2ln)p+l(n^2+(d+ e)h+(-d- e)f) +m(2ln-2fn)-2hm^2) +b(gp^2+(2gn-4lm)p-gn^2+m(2ln-2gn)+2lm^2+(-d- e)gh +(d+ e)fg)) q +a((lm-gn)p^2+(2lmn+(-h-f)m^2+( e-d)l^2+dgh- efg)p +m(gn^2+l(-n^2+(-d- e)h+(d+ e)f)- el^2 + egh)+m^2(fn-2ln)+dl^2n-dfgn +hm^3) +c^2(np^2+( ef-dh)p+m(-n^2- eh)+dfn) +bc (-mp^2+((2d-2 e)l-2mn)p+m(n^2+2 el+(d+ e)h+(-d- e)f) +2m^2n-2dln) +b^2((2m^2+( e-d)g)p-m^2n+dgn-m^3- egm))\nonumber\\ 
\delta_{1}&=\frac{-1}{\Delta}((l(fn-hn)+(h-f)lm)q^2 +(b(-2lp^2+(3ln+lm)p+l(-n^2+(-2d-2 e)h+(2d+2 e)f) +m(-ln+hn-fn)+(f-h)m^2) +c((h+f)p^2+(-hn-2fn-hm)p+hn^2+fmn+(d+ e)h^2 +(-d- e)f^2)) q +a(lp^3+((-h-f)m-ln)p^2 +(m(-ln+hn+2fn)+hm^2+((d+ e)h+(-d- e)f)l)p +m(l(n^2+ eh- ef)-hn^2+(-d- e)h^2+(d+ e)f^2) +l(dhn-dfn)-fm^2n) +bc (-p^3+np^2+(mn+(-d- e)h+(d+ e)f)p+m(-n^2- eh+ ef)-dhn +dfn) +b^2(2mp^2+(-3mn-m^2)p+m(n^2+(2d+2 e)h+(-2d-2 e)f) +m^2n)) \nonumber\\ 
\epsilon_{1}&=\frac{1}{\Delta} (((2h-2f)l^2-gh^2+f^2g)q^2 +(c((2f-2h)lp+l(2fn-2hn)+(2h^2-2f^2)m) +b((2gh-2fg)p+2ghn-2fgn+(4f-4h)lm)) q +a((l^2-gh)p^2+(-2l^2n+2fgn+(2h-2f)lm)p +l^2(n^2+2 eh-2 ef)-ghn^2+lm(2hn-2fn) +(f^2-h^2)m^2- egh^2+ ef^2g) +bc (-2lp^2+(4ln+(2f-2h)m)p+l(-2n^2-4 eh+4 ef) +m(2fn-2hn)) +c^2(hp^2-2fnp+hn^2+ eh^2- ef^2) +b^2(gp^2-2gnp+gn^2+(2h-2f)m^2+2 egh-2 efg)) \nonumber\\
\theta_{1}&=1\nonumber
\end{align}

\item
$w_{2}=\{\alpha_{1}\,,\beta_{1}\,,\gamma_{1}\,,\delta_{1}\,,\epsilon_{1}\,,1\}$
\begin{align}
\Delta&=(((2h-2f)l^2-gh^2+f^2g)q^2 +a((l^2-fg)p^2+((2gh-2l^2)n+l(2fm-2hm))p+(l^2-fg)n^2 +l(2fm-2hm)n+h^2(m^2-dg)+f^2(dg-m^2) +(2dh-2df)l^2) +bc (-2lp^2+(4ln+2hm-2fm)p-2ln^2+(2hm-2fm)n +(4df-4dh)l) +b^2(gp^2-2gnp+gn^2+f(2m^2-2dg)+h(2dg-2m^2)) +c^2(fp^2-2hnp+fn^2+dh^2-df^2))\nonumber
\end{align}

\begin{align}
A&=(2l^2-gh-fg)\nonumber\\
B&=\nonumber\\
C&=\nonumber\\
D&=\nonumber\\
E&=\nonumber\\
F&=\nonumber\\
G&=\nonumber\\
H&=\nonumber
\end{align}

\begin{align}
\alpha&=\frac{ -((Ap^2+(-4l^2+2gh+2fg)np +An^2 +((2d+2 e)h+(-2d-2 e)f)l^2 +(-d- e)gh^2+(d+ e)f^2g) q +c(-lp^3+(ln+hm+fm)p^2 +(ln^2+(-2hm-2fm)n+((-d- e)h+(d+ e)f)l)p-ln^3 +(hm+fm)n^2+((-d- e)h+(d+ e)f)ln+(d+ e)h^2m +(-d- e)f^2m) +b(gp^3+(-gn-2lm)p^2+(-gn^2+4lmn+(d+ e)gh+(-d- e)fg)p +gn^3-2lmn^2+((d+ e)gh+(-d- e)fg)n +l((-2d-2 e)hm+(2d+2 e)fm))) }{\Delta}\nonumber\\ 
\beta&=\frac{ -((Ap+(-2l^2+gh+fg)n)q^2 +(c(-lp^2+2lnp-ln^2+((-d- e)h+(d+ e)f)l) +b(gp^2-2gnp+gn^2+(d+ e)gh+(-d- e)fg)) q +a((gn-lm)p^2+(-2lmn+h(m^2-dg)+f(m^2+ eg)+(d- e)l^2)p -gn^3+3lmn^2 +(f(dg-m^2)+h(-m^2- eg)+( e-d)l^2)n +l((d+ e)hm+(-d- e)fm)) +c^2(-np^2+(dh- ef)p+n^3+( eh-df)n) +bc (mp^2+(2mn+(2 e-2d)l)p-3mn^2+(2d-2 e)ln+(-d- e)hm +(d+ e)fm)+b^2(((d- e)g-2m^2)p+(2m^2+( e-d)g)n)) }{\Delta}\nonumber\\ 
\gamma&=\frac{ ((Ap+(-2l^2+gh+fg)n)q^2 +(c(lp^2-2lnp+ln^2+((d+ e)h+(-d- e)f)l) +b(-gp^2+2gnp-gn^2+(-d- e)gh+(d+ e)fg)) q +a(gp^3-3lmp^2 +(-gn^2+2lmn+f(m^2-dg)+h(m^2+ eg)+(d- e)l^2)p +lmn^2+(h(dg-m^2)+f(-m^2- eg)+( e-d)l^2)n +l((-d- e)hm+(d+ e)fm)) +c^2(-p^3+(n^2- eh+df)p+( ef-dh)n) +bc (3mp^2+((2 e-2d)l-2mn)p-mn^2+(2d-2 e)ln+(d+ e)hm +(-d- e)fm) +b^2(((d- e)g-2m^2)p+(2m^2+( e-d)g)n)) }{\Delta}\nonumber\\ 
\delta&=\frac{ -((b(-2lp^2+4lnp-2ln^2+((-2d-2 e)h+(2d+2 e)f)l) +c((h+f)p^2+(-2h-2f)np+(h+f)n^2+(d+ e)h^2+(-d- e)f^2)) q +a(lp^3+(-ln-hm-fm)p^2 +(-ln^2+(2hm+2fm)n+((d+ e)h+(-d- e)f)l)p+ln^3 +(-hm-fm)n^2+((d+ e)h+(-d- e)f)ln+(-d- e)h^2m +(d+ e)f^2m) +bc (-p^3+np^2+(n^2+(-d- e)h+(d+ e)f)p-n^3 +((-d- e)h+(d+ e)f)n) +b^2(2mp^2-4mnp+2mn^2+(2d+2 e)hm+(-2d-2 e)fm)) }{\Delta}\nonumber\\ 
\epsilon&=1\nonumber\\
\theta&=\frac{ (((2h-2f)l^2-gh^2+f^2g)q^2 +a((gh-l^2)p^2+((2l^2-2fg)n+l(2fm-2hm))p+(gh-l^2)n^2 +l(2fm-2hm)n+h^2(m^2+ eg)+f^2(-m^2- eg) +(2 ef-2 eh)l^2) +bc (2lp^2+(-4ln+2hm-2fm)p+2ln^2+(2hm-2fm)n +(4 eh-4 ef)l) +c^2(-hp^2+2fnp-hn^2- eh^2+ ef^2) +b^2(-gp^2+2gnp-gn^2+f(2m^2+2 eg)+h(-2m^2-2 eg))) }{\Delta}\nonumber
\end{align}

\item
$w_{3}=\{\alpha_{1}\,,\beta_{1}\,,\gamma_{1}\,,\delta_{1}\,,\epsilon_{1}\,,1\}$
\begin{align}
\Delta&=(2h+2(f-\omega^{2}))q^2+b(-4p-4n)q+(a-\omega^{2})(p^2+2np+n^2+( e-(d-\omega^{2}))h\nonumber\\
&+( e-(d-\omega^{2}))(f-\omega^{2})) +b^2(2(d-\omega^{2})-2 e)\nonumber
\end{align}
\begin{align}
A&=(2lp+2ln-2hm-2(f-\omega^{2})m)\nonumber\\
B&=(-p^2-2np-n^2+((d-\omega^{2})- e)h+((d-\omega^{2})- e)(f-\omega^{2}))\nonumber\\
C&=(2mp+2mn+(2 e-2(d-\omega^{2}))\nonumber\\
D&=(2lq^2+(c(-p-n)-2bm)\nonumber\\
E&=(mp+mn+( e-(d-\omega^{2}))l)\nonumber\\
F&=(d-\omega^{2})-e\nonumber\\
G&=(c(h+(f-\omega^{2}))-2bl)\nonumber\\
H&=(lp+ln-hm-(f-\omega^{2})m)\nonumber\\
L&=(-p-n)\nonumber
\end{align}
\begin{align}
\alpha&=\frac{qA+cB +bC}{\Delta}\nonumber\\
\beta&=\gamma=\frac{-Dq+(a-\omega^{2})E+bcF}{\Delta} \nonumber\\
\delta&=1 \nonumber\\
\epsilon&=-\theta=-\frac{(Gq+(a-\omega^{2})H+bcL+2b^2m)}{\Delta} \nonumber
\end{align}

\item
$w_{4}=\{\alpha_{1}\,,\beta_{1}\,,\gamma_{1}\,,\delta_{1}\,,\epsilon_{1}\,,1\}$
\begin{align}
\Delta&=((gp^2-2gnp+gn^2+(2d+2 e)l^2+(-2d-2 e)fg)q^2 +(c(-2mp^2+(4mn+(-2d-2 e)l)p-2mn^2+(-2d-2 e)ln +(4d+4 e)fm) +b((2d+2 e)gp+(2d+2 e)gn+(-4d-4 e)lm)) q +a((m^2-dg)p^2+((-2m^2-2 eg)n+(2d+2 e)lm)p +(m^2-dg)n^2+(2d+2 e)lmn +f((-2d-2 e)m^2+(d^2- e^2)g)+( e^2-d^2)l^2) +c^2(dp^2+2 enp+dn^2+( e^2-d^2)f) +bc((-2d-2 e)mp+(-2d-2 e)mn+(2d^2-2 e^2)l) +b^2((2d+2 e)m^2+( e^2-d^2)g))\nonumber
\end{align}

\begin{align}
A&=(2l^2-gh-fg)\nonumber\\
B&=\nonumber\\
C&=\nonumber\\
D&=\nonumber\\
E&=\nonumber\\
F&=\nonumber\\
G&=\nonumber\\
H&=\nonumber
\end{align}

\begin{align}
\alpha&=\frac{1}{\Delta}(-((gp^3+(-gn-2lm)p^2 +(-gn^2+4lmn+(d+ e)gh+(-d- e)fg)p+gn^3-2lmn^2\nonumber\\
& +((d+ e)gh+(-d- e)fg)n +l((-2d-2 e)hm+(2d+2 e)fm)) q \nonumber\\
&+c(-mp^3+(mn+(d- e)l)p^2 +(mn^2+(2 e-2d)ln+(-d- e)hm+(d+ e)fm)p\nonumber\\
&-mn^3 +(d- e)ln^2+((-d- e)hm+(d+ e)fm)n +((d^2- e^2)h+( e^2-d^2)f)l)\nonumber\\
& +b((2m^2+( e-d)g)p^2+((2d-2 e)g-4m^2)np +(2m^2+( e-d)g)n^2\nonumber\\
& +h((2d+2 e)m^2+( e^2-d^2)g) +f((-2d-2 e)m^2+(d^2- e^2)g))))\nonumber\\
\beta&=\frac{1}{\Delta}(((gp^2-2gnp+gn^2+(-2d-2 e)l^2+(2d+2 e)gh)q^2 \nonumber\\
&+(c(-2mp^2+(4mn+(2d+2 e)l)p-2mn^2+(2d+2 e)ln +(-4d-4 e)hm)\nonumber\\
& +b((-2d-2 e)gp+(-2d-2 e)gn+(4d+4 e)lm)) q +a((m^2+ eg)p^2\nonumber\\
&+((2dg-2m^2)n+(-2d-2 e)lm)p +(m^2+ eg)n^2+(-2d-2 e)lmn \nonumber\\
&+h((2d+2 e)m^2+( e^2-d^2)g)+(d^2- e^2)l^2) +c^2(- ep^2-2dnp- en^2+(d^2- e^2)h)\nonumber\\
& +bc((2d+2 e)mp+(2d+2 e)mn+(2 e^2-2d^2)l) +b^2((-2d-2 e)m^2+(d^2- e^2)g)))\nonumber\\
\gamma&=1\nonumber\\
\delta&=\frac{1}{\Delta}(-((2lp^2-4lnp+2ln^2+((2d+2 e)h+(-2d-2 e)f)l)q^2\nonumber\\
& +(c(-p^3+np^2+(n^2+(-d- e)h+(d+ e)f)p-n^3 +((-d- e)h+(d+ e)f)n)\nonumber\\
& +b(-2mp^2+4mnp-2mn^2+(-2d-2 e)hm+(2d+2 e)fm)) q +a(mp^3+(( e-d)l-mn)p^2\nonumber\\
& +(-mn^2+(2d-2 e)ln+(d+ e)hm+(-d- e)fm)p+mn^3 +( e-d)ln^2\nonumber\\
&+((d+ e)hm+(-d- e)fm)n +(( e^2-d^2)h+(d^2- e^2)f)l) +bc ((d- e)p^2\nonumber\\
&+(2 e-2d)np+(d- e)n^2+(d^2- e^2)h+( e^2-d^2)f)))\nonumber\\
\epsilon&=\frac{1}{\Delta}(-((Ap+(-2l^2+gh+fg)n)q^2\nonumber\\
& +(c(-3lp^2+(2ln+2hm+2fm)p+ln^2+(-2hm-2fm)n +((-d- e)h+(d+ e)f)l)\nonumber\\
& +b(3gp^2+(-2gn-4lm)p-gn^2+4lmn+(d+ e)gh+(-d- e)fg)) q \nonumber\\
&+a(-gp^3+3lmp^2 +(gn^2-2lmn+f(dg-m^2)+h(-m^2- eg)+( e-d)l^2)p\nonumber\\
& -lmn^2+(h(m^2-dg)+f(m^2+ eg)+(d- e)l^2)n +l((d+ e)hm+(-d- e)fm))\nonumber\\
& +c^2(p^3+(-n^2+ eh-df)p+(dh- ef)n) +bc (-3mp^2+(2mn+(2d-2 e)l)p+mn^2\nonumber\\
&+(2 e-2d)ln+(-d- e)hm +(d+ e)fm) +b^2((2m^2+( e-d)g)p+((d- e)g-2m^2)n)))\nonumber\\
\theta&=\frac{1}{\Delta}(-((Ap+(-2l^2+gh+fg)n)q^2\nonumber\\
& +(c(-lp^2+(-2ln+2hm+2fm)p+3ln^2+(-2hm-2fm)n +((d+ e)h+(-d- e)f)l)\nonumber\\
& +b(gp^2+(2gn-4lm)p-3gn^2+4lmn+(-d- e)gh+(d+ e)fg)) q \nonumber\\
&+a((lm-gn)p^2+(2lmn+h(dg-m^2)+f(-m^2- eg)+( e-d)l^2)p +gn^3\nonumber\\
&-3lmn^2 +(f(m^2-dg)+h(m^2+ eg)+(d- e)l^2)n +l((-d- e)hm+(d+ e)fm))\nonumber\\
& +c^2(np^2+( ef-dh)p-n^3+(df- eh)n) +bc (-mp^2+((2d-2 e)l-2mn)p+3mn^2\nonumber\\
&+(2 e-2d)ln+(d+ e)hm +(-d- e)fm)+b^2((2m^2+( e-d)g)p+((d- e)g-2m^2)n)))\nonumber
\end{align}

\item
$w_{5}=\{\alpha_{1}\,,\beta_{1}\,,\gamma_{1}\,,\delta_{1}\,,\epsilon_{1}\,,1\}$
\begin{align}
\Delta&=((gp^2-2gnp+gn^2+(2d+2 e)l^2+(-2d-2 e)fg)q^2 +(c(-2mp^2+(4mn+(-2d-2 e)l)p-2mn^2+(-2d-2 e)ln +(4d+4 e)fm) +b((2d+2 e)gp+(2d+2 e)gn+(-4d-4 e)lm)) q +a((m^2-dg)p^2+((-2m^2-2 eg)n+(2d+2 e)lm)p +(m^2-dg)n^2+(2d+2 e)lmn +f((-2d-2 e)m^2+(d^2- e^2)g)+( e^2-d^2)l^2) +c^2(dp^2+2 enp+dn^2+( e^2-d^2)f) +bc((-2d-2 e)mp+(-2d-2 e)mn+(2d^2-2 e^2)l) +b^2((2d+2 e)m^2+( e^2-d^2)g))\nonumber
\end{align}

\begin{align}
A&=(2l^2-gh-fg)\nonumber\\
B&=\nonumber\\
C&=\nonumber\\
D&=\nonumber\\
E&=\nonumber\\
F&=\nonumber\\
G&=\nonumber\\
H&=\nonumber
\end{align}
\begin{align}
\alpha &=\frac{ -((gp^3+(-gn-2lm)p^2 +(-gn^2+4lmn+(d+ e)gh+(-d- e)fg)p+gn^3-2lmn^2 +((d+ e)gh+(-d- e)fg)n +l((-2d-2 e)hm+(2d+2 e)fm)) q +c(-mp^3+(mn+(d- e)l)p^2 +(mn^2+(2 e-2d)ln+(-d- e)hm+(d+ e)fm)p-mn^3 +(d- e)ln^2+((-d- e)hm+(d+ e)fm)n +((d^2- e^2)h+( e^2-d^2)f)l) +b((2m^2+( e-d)g)p^2+((2d-2 e)g-4m^2)np +(2m^2+( e-d)g)n^2 +h((2d+2 e)m^2+( e^2-d^2)g) +f((-2d-2 e)m^2+(d^2- e^2)g))) }{\Delta}\nonumber\\ 
\beta&=1\nonumber\\
\gamma &=\frac{ ((gp^2-2gnp+gn^2+(-2d-2 e)l^2+(2d+2 e)gh)q^2 +(c(-2mp^2+(4mn+(2d+2 e)l)p-2mn^2+(2d+2 e)ln +(-4d-4 e)hm) +b((-2d-2 e)gp+(-2d-2 e)gn+(4d+4 e)lm)) q +a((m^2+ eg)p^2+((2dg-2m^2)n+(-2d-2 e)lm)p +(m^2+ eg)n^2+(-2d-2 e)lmn +h((2d+2 e)m^2+( e^2-d^2)g)+(d^2- e^2)l^2) +c^2(- ep^2-2dnp- en^2+(d^2- e^2)h) +bc((2d+2 e)mp+(2d+2 e)mn+(2 e^2-2d^2)l) +b^2((-2d-2 e)m^2+(d^2- e^2)g)) }{\Delta}\nonumber\\ 
\delta &= \frac{-((2lp^2-4lnp+2ln^2+((2d+2 e)h+(-2d-2 e)f)l)q^2 +(c(-p^3+np^2+(n^2+(-d- e)h+(d+ e)f)p-n^3 +((-d- e)h+(d+ e)f)n) +b(-2mp^2+4mnp-2mn^2+(-2d-2 e)hm+(2d+2 e)fm)) q +a(mp^3+(( e-d)l-mn)p^2 +(-mn^2+(2d-2 e)ln+(d+ e)hm+(-d- e)fm)p+mn^3 +( e-d)ln^2+((d+ e)hm+(-d- e)fm)n +(( e^2-d^2)h+(d^2- e^2)f)l) +bc ((d- e)p^2+(2 e-2d)np+(d- e)n^2+(d^2- e^2)h+( e^2-d^2)f)) }{\Delta}\nonumber\\ 
\epsilon &=\frac{ ((Ap+(-2l^2+gh+fg)n)q^2 +(c(-lp^2+(-2ln+2hm+2fm)p+3ln^2+(-2hm-2fm)n +((d+ e)h+(-d- e)f)l) +b(gp^2+(2gn-4lm)p-3gn^2+4lmn+(-d- e)gh+(d+ e)fg)) q +a((lm-gn)p^2+(2lmn+h(dg-m^2)+f(-m^2- eg)+( e-d)l^2)p +gn^3-3lmn^2 +(f(m^2-dg)+h(m^2+ eg)+(d- e)l^2)n +l((-d- e)hm+(d+ e)fm)) +c^2(np^2+( ef-dh)p-n^3+(df- eh)n) +bc (-mp^2+((2d-2 e)l-2mn)p+3mn^2+(2 e-2d)ln+(d+ e)hm +(-d- e)fm)+b^2((2m^2+( e-d)g)p+((d- e)g-2m^2)n)) }{\Delta}\nonumber\\ 
\theta &=\frac{ ((Ap+(-2l^2+gh+fg)n)q^2 +(c(-3lp^2+(2ln+2hm+2fm)p+ln^2+(-2hm-2fm)n +((-d- e)h+(d+ e)f)l) +b(3gp^2+(-2gn-4lm)p-gn^2+4lmn+(d+ e)gh+(-d- e)fg)) q +a(-gp^3+3lmp^2 +(gn^2-2lmn+f(dg-m^2)+h(-m^2- eg)+( e-d)l^2)p -lmn^2+(h(m^2-dg)+f(m^2+ eg)+(d- e)l^2)n +l((d+ e)hm+(-d- e)fm)) +c^2(p^3+(-n^2+ eh-df)p+(dh- ef)n) +bc (-3mp^2+(2mn+(2d-2 e)l)p+mn^2+(2 e-2d)ln+(-d- e)hm +(d+ e)fm) +b^2((2m^2+( e-d)g)p+((d- e)g-2m^2)n)) }{\Delta}\nonumber
\end{align}

\item
$w_{6}=\{1\,,\beta_{6}\,,\gamma_{6}\,,\delta_{6}\,,\epsilon_{6}\,,\theta_{6}\}$
\begin{align}
\Delta&=g(p+n)^2+(h+f)(2m^2+( e-d)g)+2(d-e)l^2-4lm(n+p)\,,\nonumber
\end{align}

\begin{align}
\alpha&=1\nonumber\\
\beta&=\gamma=\frac{l(2mq+c( e-d))+(p+n)(cm-gq)+b((d- e)g-2m^{2})}{\Delta}\nonumber\\
\delta& =-\frac{(f+h)(2mq+c( e-d))-2(p+n)(lq+bm)+c(p+n)^2+2bl(d-e)}{\Delta}\nonumber\\
\epsilon&=-\theta=\frac{(h+f)(gq-cm)+(cl-bg)(p+n)+2l(bm-lq)}{\Delta}\nonumber
\end{align}
\end{itemize}
