# Supplementary material for: Wave propagation in micromorphic anisotropic continua with an application to tetragonal crystals
Source: arXiv:2009.09825 source file (2020-09-21)
Supplement: Supplementary file 2 [file appendix.tex]

\section{Appendix}

\subsection{The fourth-order inertia tensor}

Let $\Jb$ be the micro-inertia tensor whose components are $J_{ij}=J_{ji}$, $i,j=1,2,3$. Then, by (\ref{componentsHO})$_{5}$, the matrix of $\Jel$ is\footnote{We use the Voigt notation for fourth-order tensors which maps $\Lin$ into itself namely $1=11\,,2=22\,,3=33$, $4=23\,,5=31\,,6=12$, $7=32\,,8=13\,,9=21$. For mappings from and into $\Sym$ we have $4=23=32$, $5=13=31$ and $6=12=21$.}
\begin{equation}\label{Jfourth1}
[\Jel]\equiv
\left[
\begin{array}{ccccccccc}
J_{11}  & 0  & 0 & 0 & 0  & J_{12} &0 & J_{13} & 0\\
0  & J_{22}  & 0 & J_{23} & 0  & 0 &0&0&J_{12} \\
0   & 0  & J_{33} & 0 & J_{13}  & 0&J_{23}&0&0\\
0   &  0  & J_{23} & 0 &J_{12} & 0 &J_{22}&0&0\\
J_{13}  &  0  & 0 & 0  & 0 & J_{23}&0&J_{33}&0 \\
0  & J_{12}   & 0  & 0  & 0  & 0&0&J_{23}&J_{11}  \\
0 & J_{23} &0 & J_{33} & 0&0 &0&0&J_{13}\\
0  &  0  & J_{13}  & 0  & J_{11}  & 0 &J_{12} &0&0\\
J_{12}  & 0 & 0 & 0  & 0  & J_{22} &0 & J_{23} &0\\
 \end{array}
\right]\,.
\end{equation}

For tetragonal crystals, provided we identify the $c-$axis with the direction $\eb_{3}$, we have $J_{11}=J_{22}$ and $J_{ij}=0\,,i\neq j$: accordingly (\ref{Jfourth1}) reduces to:
\begin{equation}\label{Jtetra}
[\Jel]\equiv
\left[
\begin{array}{ccccccccc}
J_{11}  & 0  & 0 & 0 & 0  & 0 &0&0&0\\
0  & J_{11}  & 0 & 0 & 0  & 0 &0&0&0 \\
0   & 0  & J_{33} & 0 & 0  & 0&0&0&0\\
0   &  0  & 0 & 0 &0 & 0 &J_{11}&0&0\\
0  &  0  & 0 & 0  & 0 & 0&0&J_{33}&0 \\
0  & 0   & 0  & 0  & 0  & 0&0&0&J_{11}  \\
0 & 0 &0 & J_{33} & 0&0 &0&0&0\\
0  &  0  & 0  & 0  & J_{11}  & 0 &0 &0&0\\
0  & 0 & 0 & 0  &0  & J_{11} &0 & 0 &0\\
 \end{array}
\right]\,.
\end{equation}

\subsection{The fourth-order tensors}

The non-zero components for all the classes of the Tetragonal point group are given in tabular form into \cite{AU03} for the tensors $\Cel$ and $\Bel$ whereas those of $\Del$ can be obtained from those of $\Bel$ with the additional conditions induced by the symmetries of the first two components. The elasticity tensor $\Cel$ for tetragonal crystals (all classes) has 6 independent components. As far as the other two fourth-order tensors we have, for the low-symmetry classes $4\,,\bar{4}$ and $4/m$ we have
\begin{itemize}
\item $\Bel$: 13 components,
\item $\Del$: 16 components;
\end{itemize}
whereas for the high-symmetry classes $4mm\,,422\,,\bar{4}2m$ and $4/mm$ we have:
\begin{itemize}
\item $\Bel$: 10 components,
\item $\Del$: 8 components.
\end{itemize}

\subsubsection{The elasticity tensor $\Cel$}

All classes:

\begin{equation}\label{tetraC}
[\Cel]\equiv
\left[
\begin{array}{cccccc}
\Cel_{1111}  & \Cel_{1122}  & \Cel_{1133} & 0 & 0  & 0 \\
\cdot  & \Cel_{1111}  & \Cel_{1133} & 0 & 0  & 0 \\
\cdot  & \cdot & \Cel_{3333} & 0 & 0  & 0\\
\cdot &  \cdot & \cdot & \Cel_{2323} & 0 & 0 \\
\cdot &  \cdot & \cdot & \cdot & \Cel_{2323} & 0 \\
\cdot & \cdot  & \cdot & \cdot & \cdot  & \Cel_{1212}   
 \end{array}
\right]\,;
\end{equation}

\subsubsection{The tensor $\Del$}

Classes $4$, $\bar{4}$ and $4/m$:

\begin{equation}
[\Del]\equiv
\left[
\begin{array}{ccccccccc}
\Del_{1111}  & \Del_{1122}  & \Del_{1133} & 0 & 0  & \Del_{1112} &0&0&-\Del_{2212}\\
\Del_{1122}  & \Del_{1111}  & \Del_{1133} & 0 & 0  & \Del_{2212}&0&0&-\Del_{1112} \\
\Del_{3311}  & \Del_{3311}  & \Del_{3333} & 0 & 0  & \Del_{3312}&0&0&-\Del_{3312}\\
0  &  0 & 0 & \Del_{2323} & \Del_{2331} & 0 &\Del_{3131}&-\Del_{3123}&0\\
0  &  0 & 0 & \Del_{3123} & \Del_{3131} & 0&-\Del_{2331}&\Del_{2323}&0 \\
\Del_{1211}  & -\Del_{1211}  & 0& 0 & 0  & \Del_{1212}&0&0&\Del_{1212}  \\ 
 \end{array}
\right]\,;
\end{equation}

Classes $4mmm$, $422$, $4/mm$  and $\bar{4}2m$: 

\begin{equation}
[\Del]\equiv
\left[
\begin{array}{ccccccccc}
\Del_{1111}  & \Del_{1122}  & \Del_{1133} & 0 & 0  & 0 &0&0&0\\
\Del_{1122}  & \Del_{1111}  & \Del_{1133} & 0 & 0  & 0&0&0&0 \\
\Del_{3311}  & \Del_{3311}  & \Del_{3333} & 0 & 0  & 0&0&0&0\\
0  &  0 & 0 & \Del_{2323} & 0 & 0 &\Del_{3131}&0&0\\
0  &  0 & 0 & 0 & \Del_{3131} & 0&0&\Del_{2323}&0 \\
0  &0  & 0 & 0 & 0  & \Del_{1212}&0&0&\Del_{1212}  \\ 
 \end{array}
\right]\,;
\end{equation}

\subsubsection{The tensor $\Bel$}

Classes $4$, $\bar{4}$ and $4/m$:

\begin{equation}\label{BtensorLS}
[\Bel]\equiv
\left[
\begin{array}{ccccccccc}
\Bel_{1111}  & \Bel_{1122}  & \Bel_{1133} & 0 & 0  & \Bel_{1112} &0&0&-\Bel_{2212}\\
\cdot  & \Bel_{1111}  & \Bel_{1133} & 0 & 0  & \Bel_{2212}&0&0&-\Bel_{1112} \\
\cdot   & \cdot   & \Bel_{3333} & 0 & 0  & \Bel_{3312}&0&0&-\Bel_{3312}\\
\cdot   &  \cdot  & \cdot  & \Bel_{2323} & \Bel_{2331} & 0 &\Bel_{2332}&0&0\\
\cdot  &  \cdot  & \cdot  & \cdot  & \Bel_{3131} & 0&0&\Bel_{2332}&0 \\
\cdot   & \cdot   & \cdot  & \cdot  & \cdot   & \Bel_{1212}&0&0&\Bel_{1221}  \\
 \cdot &\cdot &\cdot & \cdot  & \cdot &\cdot &\Bel_{3131}&-\Bel_{2331}&0\\
\cdot  &  \cdot  & \cdot  & \cdot  & \cdot  & \cdot  &\cdot &\Bel_{2323}&0\\
\cdot   &  \cdot  & \cdot & \cdot  & \cdot  & \cdot & \cdot & \cdot &\Bel_{1212}\\
  \end{array}
\right]\,;
\end{equation}

Classes $4mmm$, $422$, $4/mm$  and $\bar{4}2m$:

\begin{equation}
[\Bel]\equiv
\left[
\begin{array}{ccccccccc}
\Bel_{1111}  & \Bel_{1122}  & \Bel_{1133} & 0 & 0  & 0 &0&0&0\\
\cdot  & \Bel_{1111}  & \Bel_{1133} & 0 & 0  &0&0&0&0 \\
\cdot   & \cdot   & \Bel_{3333} & 0 & 0  & 0&0&0&0\\
\cdot   &  \cdot  & \cdot  & \Bel_{2323} & 0 & 0 &\Bel_{2332}&0&0\\
\cdot  &  \cdot  & \cdot  & \cdot  & \Bel_{3131} & 0&0&\Bel_{2332}&0 \\
\cdot   & \cdot   & \cdot  & \cdot  & \cdot   & \Bel_{1212}&0&0&\Bel_{1221}  \\
 \cdot &\cdot &\cdot & \cdot  & \cdot &\cdot &\Bel_{3131}&0&0\\
\cdot  &  \cdot  & \cdot  & \cdot  & \cdot  & \cdot  &\cdot &\Bel_{2323}&0\\
\cdot   &  \cdot  & \cdot & \cdot  & \cdot  & \cdot & \cdot & \cdot &\Bel_{1212}\\
  \end{array}
\right]\,;
\end{equation}

\subsection{The fifth- and  sixth-order tensors}

A detailed study of the symmetries for fifth- and sixth-order tensor was done into \cite{FIFU53}: the more recent results obtained into [] cannot be applied to the present case since they apply to tensors endowed with some minor symmetries which in our case are missing. For the Tetragonal group the symmetries are different between classes, and accordingly we study them in detail beginning with the fifth-order tensor $\caG$. We follow \cite{FIFU53} into the use of the notation
\begin{equation}
\caG_{11112}\,,\quad (5)\,,
\end{equation}
to denote all the 5 possible combinations of the index, namely: $\caG_{11112}$, $\caG_{11121}$, $\caG_{11211}$, $\caG_{12111}$ and $\caG_{21111}$.

\subsubsection{Class $4$}

For the this class the non null components are
\begin{eqnarray}\label{caG1}
&\caG_{33333}\,,\quad (1)\,,\nonumber\\
&\caG_{11113}=\caG_{22223}\,,\quad (5)\,,\nonumber\\
&\caG_{11333}=\caG_{22333}\,,\quad (10)\,,\nonumber\\
&\caG_{11123}=-\caG_{22213}\,,\quad (20)\,,\\
&\caG_{33312}=-\caG_{33321}\,,\quad (10)\,,\nonumber\\
&\caG_{11223}=\caG_{22113}\,,\quad (15)\,,\nonumber
\end{eqnarray}
which gives a total of 61 independent components, which in explicit read:
\begin{equation}\label{noPWO1}
\caG_{33333}\,,
\end{equation}
\begin{eqnarray}
&\caG_{11113}=\caG_{22223}\,,\nonumber\\
&\caG_{11131}=\caG_{22232}\,,\nonumber\\
&\caG_{11311}=\caG_{22322}\,,\\
&\caG_{13111}=\caG_{23222}\,,\nonumber\\
&\caG_{31111}=\caG_{32222}\,,\nonumber
\end{eqnarray}
\begin{eqnarray}
&\caG_{11333}=\caG_{22333}\,,\nonumber\\
&\caG_{31133}=\caG_{32233}\,,\nonumber\\
&\caG_{33113}=\caG_{33223}\,,\nonumber\\
&\caG_{33311}=\caG_{33322}\,,\nonumber\\
&\caG_{13133}=\caG_{23233}\,,\\
&\caG_{13313}=\caG_{23323}\,,\nonumber\\
&\caG_{13331}=\caG_{23332}\,,\nonumber\\
&\caG_{31313}=\caG_{32323}\,,\nonumber\\
&\caG_{31331}=\caG_{32333}\,,\nonumber\\
&\caG_{33131}=\caG_{33232}\,,\nonumber
\end{eqnarray}
\begin{eqnarray}
&\caG_{23111}=\caG_{13222}\,,\nonumber\\
&\caG_{12311}=\caG_{21322}\,,\nonumber\\
&\caG_{11231}=\caG_{22132}\,,\nonumber\\
&\caG_{11123}=\caG_{22213}\,,\nonumber\\
&\caG_{21311}=\caG_{12322}\,,\nonumber\\
&\caG_{21131}=\caG_{12232}\,,\nonumber\\
&\caG_{21113}=\caG_{12223}\,,\nonumber\\
&\caG_{12131}=\caG_{21232}\,,\nonumber\\
&\caG_{12113}=\caG_{21223}\,,\nonumber\\
&\caG_{11213}=\caG_{22123}\,,\\
&\caG_{32111}=\caG_{31222}\,,\nonumber\\
&\caG_{13211}=\caG_{23122}\,,\nonumber\\
&\caG_{11321}=\caG_{22312}\,,\nonumber\\
&\caG_{11132}=\caG_{22231}\,,\nonumber\\
&\caG_{31211}=\caG_{32122}\,,\nonumber\\
&\caG_{31121}=\caG_{32212}\,,\nonumber\\
&\caG_{31112}=\caG_{32221}\,,\nonumber\\
&\caG_{13121}=\caG_{23212}\,,\nonumber\\
&\caG_{13112}=\caG_{23221}\,,\nonumber\\
&\caG_{11312}=\caG_{22321}\,,\nonumber
\end{eqnarray}
\begin{eqnarray}\label{noPWO2}
&\caG_{12333}=-\caG_{21333}\,,\nonumber\\
&\caG_{31233}=-\caG_{32133}\,,\nonumber\\
&\caG_{33123}=-\caG_{33213}\,,\nonumber\\
&\caG_{33312}=-\caG_{33321}\,,\nonumber\\
&\caG_{13233}=-\caG_{23133}\,,\nonumber\\
&\caG_{13323}=-\caG_{23313}\,,\\
&\caG_{13332}=-\caG_{23331}\,,\nonumber\\
&\caG_{31323}=-\caG_{32313}\,,\nonumber\\
&\caG_{31332}=-\caG_{32331}\,,\nonumber\\
&\caG_{33132}=-\caG_{33231}\,,\nonumber
\end{eqnarray}
\begin{eqnarray}
&\caG_{11223}=\caG_{22113}\,,\nonumber\\
&\caG_{11232}=\caG_{22131}\,,\nonumber\\
&\caG_{11322}=\caG_{22311}\,,\nonumber\\
&\caG_{21123}=\caG_{12213}\,,\nonumber\\
&\caG_{21132}=\caG_{12231}\,,\nonumber\\
&\caG_{31122}=\caG_{32211}\,,\nonumber\\
&\caG_{23112}=\caG_{13221}\,,\nonumber\\
&\caG_{32112}=\caG_{31221}\,,\\
&\caG_{23211}=\caG_{13122}\,,\nonumber\\
&\caG_{12123}=\caG_{21213}\,,\nonumber\\
&\caG_{12132}=\caG_{21231}\,,\nonumber\\
&\caG_{12312}=\caG_{21321}\,,\nonumber\\
&\caG_{13212}=\caG_{23121}\,,\nonumber\\
&\caG_{12321}=\caG_{21312}\,,\nonumber\\
&\caG_{31221}=\caG_{32121}\,.\nonumber
\end{eqnarray}

We may find convenient to these results in a tabular form as a $9\times 9$ block matrix:
\begin{equation}
 % give some more room
\caG\equiv
\left[
\begin{array}{@{}c|c@{}|c@{}}
\caG_{1}  & \caG_{2}\, &\caG_{3} \\ 
\end{array}
\right]\,.
\end{equation}
were the three blocks are given by
\begin{equation}
\caG_{1}\equiv
\left[
\begin{array}{ccccccccc}
\caG_{11111}  & \caG_{11122}  & \caG_{11133} & \caG_{11123}&\caG_{11131} &\caG_{11112} &\caG_{11132} & \caG_{11113} & \caG_{11121}\\
\caG_{22111}  & \caG_{22122}  & \caG_{22133} & \caG_{22123}&\caG_{22131} &\caG_{22112} &\caG_{22132} & \caG_{22113} & \caG_{22121}\\
\caG_{33111}  & \caG_{33122}  & \caG_{33133} & \caG_{33123}&\caG_{33131} &\caG_{33112} &\caG_{33132} & \caG_{33113} & \caG_{33121}\\
\caG_{23111}  & \caG_{23122}  & \caG_{23133} & \caG_{23123}&\caG_{23131} &\caG_{23112} &\caG_{23132} & \caG_{23113} & \caG_{23121}\\
\caG_{31111}  & \caG_{31122}  & \caG_{31133} & \caG_{31123}&\caG_{31131} &\caG_{31112} &\caG_{31132} & \caG_{31113} & \caG_{31121}\\
\caG_{12111}  & \caG_{12122}  & \caG_{12133} & \caG_{12123}&\caG_{12131} &\caG_{12112} &\caG_{12132} & \caG_{12113} & \caG_{12121}\\
\caG_{32111}  & \caG_{32122}  & \caG_{32133} & \caG_{32123}&\caG_{32131} &\caG_{32112} &\caG_{32132} & \caG_{32113} & \caG_{32121}\\
\caG_{13111}  & \caG_{13122}  & \caG_{13133} & \caG_{13123}&\caG_{13131} &\caG_{13112} &\caG_{13132} & \caG_{13113} & \caG_{13121}\\
\caG_{21111}  & \caG_{21122}  & \caG_{21133} & \caG_{21123}&\caG_{21131} &\caG_{21112} &\caG_{21132} & \caG_{21113} & \caG_{21121}  
\end{array}
\right]
\end{equation}
\begin{equation}
\caG_{2}\equiv
\left[
\begin{array}{ccccccccc}
\caG_{11211}  & \caG_{11222}  & \caG_{11233} & \caG_{11223}&\caG_{11231} &\caG_{11212} &\caG_{11232} & \caG_{11213} & \caG_{11221}\\
\caG_{22211}  & \caG_{22222}  & \caG_{22233} & \caG_{22223}&\caG_{22231} &\caG_{22212} &\caG_{22232} & \caG_{22213} & \caG_{22221}\\
\caG_{33211}  & \caG_{33222}  & \caG_{33233} & \caG_{33223}&\caG_{33231} &\caG_{33212} &\caG_{33232} & \caG_{33213} & \caG_{33221}\\
\caG_{23211}  & \caG_{23222}  & \caG_{23233} & \caG_{23223}&\caG_{23231} &\caG_{23212} &\caG_{23232} & \caG_{23213} & \caG_{23221}\\
\caG_{31211}  & \caG_{31222}  & \caG_{31233} & \caG_{31223}&\caG_{31231} &\caG_{31212} &\caG_{31232} & \caG_{31213} & \caG_{31221}\\
\caG_{12211}  & \caG_{12222}  & \caG_{12233} & \caG_{12223}&\caG_{12231} &\caG_{12212} &\caG_{12232} & \caG_{12213} & \caG_{12221}\\
\caG_{32211}  & \caG_{32222}  & \caG_{32233} & \caG_{32223}&\caG_{32231} &\caG_{32212} &\caG_{32232} & \caG_{32213} & \caG_{32221}\\
\caG_{13211}  & \caG_{13222}  & \caG_{13233} & \caG_{13223}&\caG_{13231} &\caG_{13212} &\caG_{13232} & \caG_{13213} & \caG_{13221}\\
\caG_{21211}  & \caG_{21222}  & \caG_{21233} & \caG_{21223}&\caG_{21231} &\caG_{21212} &\caG_{21232} & \caG_{21213} & \caG_{21221} 
\end{array}
\right]
\end{equation}
\begin{equation}
\caG_{3}\equiv
\left[
\begin{array}{ccccccccc}
\caG_{11311}  & \caG_{11322}  & \caG_{11333} & \caG_{11323}&\caG_{11331} &\caG_{11312} &\caG_{11332} & \caG_{11313} & \caG_{11321}\\
\caG_{22311}  & \caG_{22322}  & \caG_{22333} & \caG_{22323}&\caG_{22331} &\caG_{22312} &\caG_{22332} & \caG_{22313} & \caG_{22321}\\
\caG_{33311}  & \caG_{33322}  & \caG_{33333} & \caG_{33323}&\caG_{33331} &\caG_{33312} &\caG_{33332} & \caG_{33313} & \caG_{33321}\\
\caG_{23311}  & \caG_{23322}  & \caG_{23333} & \caG_{23323}&\caG_{23331} &\caG_{23312} &\caG_{23332} & \caG_{23313} & \caG_{23321}\\
\caG_{31311}  & \caG_{31322}  & \caG_{31333} & \caG_{31323}&\caG_{31331} &\caG_{31312} &\caG_{31332} & \caG_{31313} & \caG_{31321}\\
\caG_{12311}  & \caG_{12322}  & \caG_{12333} & \caG_{12323}&\caG_{12331} &\caG_{12312} &\caG_{12332} & \caG_{12313} & \caG_{12321}\\
\caG_{32311}  & \caG_{32322}  & \caG_{32333} & \caG_{32323}&\caG_{32331} &\caG_{32312} &\caG_{32332} & \caG_{32313} & \caG_{32321}\\
\caG_{13311}  & \caG_{13322}  & \caG_{13333} & \caG_{13323}&\caG_{13331} &\caG_{13312} &\caG_{13332} & \caG_{13313} & \caG_{13321}\\
\caG_{21311}  & \caG_{21322}  & \caG_{21333} & \caG_{21323}&\caG_{21331} &\caG_{21312} &\caG_{21332} & \caG_{21313} & \caG_{21321}
\end{array}
\right]
\end{equation}

\subsubsection{Classes $\bar{4}$ and $4/m$}

For these classes we have the following restrictions into (\ref{caG1})
\begin{equation}\label{caG2}
\caG_{33333}=0\,,\quad\caG_{33312}=\caG_{33321}=0\,,
\end{equation}
which means that (\ref{noPWO1}) and (\ref{noPWO2}) must be zero and the independent components reduce to 50.

\subsubsection{Class $4/mm$}

For this class the tensors $\caG$ splits into a polar and an axial ones. The polar tensor ha 61 non-zero components:
\begin{eqnarray}
&\caG_{33333}\,,\quad\caG_{22223}=\caG_{11113}\,,\quad (5)\,,\\
&\caG_{33322}=\caG_{33311}\,,\quad (10)\,,\quad\caG_{22113}=\caG_{11223}\,,\quad (15)\,,\nonumber
\end{eqnarray}
31 being the independent ones, wheras the axial tensor has 60 components with only 30 independent:
\begin{equation}\label{4mmP}
\caG_{22213}=-\caG_{11123}\,,\quad (20)\,,\quad\caG_{33312}=-\caG_{33321}\,,\quad (10)\,,
\end{equation}
The components for the class $\bar{4}2m$ are obtained by chancing the sign of the components (\ref{4mmP}), whereas those for the classes $422$ and $4mmm$ are obtained by setting to zero (\ref{4mmP}).  

Finally, to obtain the number of the independent components for the tensor $\caF$, we recall that it obeys $\caF_{ijhkm}=\caF_{jihkm}$ and hence the number of independent components reduces to
\begin{itemize}
\item Class $4$:  41 components\,,
\item Class $\bar{4}$ and $4/m$: 33 components\,,
\item Classes $4/mm$, $\bar{4}2m$, $4mmm$ and $422$, Polar tensor: 42 components, (21 independent)\,.
\end{itemize}

\subsection{The sixth-order tensor $\caH$}

Also for sixth-order tensors the symmetries changes for different classes. Following \cite{FIFU53} we have that, by using the same convention of the fifth-order tensor, that the for the class $4$ the non-null components are:
\begin{eqnarray}\label{4H6nonzero}
&\caH_{111111}\,,\quad\caH_{222222}\,,\quad\caH_{333333}\,,\quad\caH_{111112}\quad(6)\,,\quad\caH_{222221}\quad(6)\,,\nonumber\\
&\caH_{111122}\quad (15)\,,\quad\caH_{222211}\quad (15)\,,\quad\caH_{111133}\quad (15)\,,\quad\caH_{222233}\quad (15)\,,\\
&\caH_{333311}\quad (15)\,,\quad\caH_{333322}\quad (15)\,,\quad\caH_{333312}\quad (30)\,,\nonumber\\
&\caH_{111222}\quad (20)\,,\quad\caH_{111332}\quad (60)\,,\quad\caH_{222331}\quad (60)\,,\quad\caH_{112233}\quad (90)\,,\nonumber
\end{eqnarray}
with the conditions:
\begin{eqnarray}\label{4H6condition}
&\caH_{111111}=\caH_{222222},,\quad\caH_{222221}=-\caH_{111112}\quad(6)\,,\nonumber\\
&\caH_{222211}=\caH_{222211}\quad(15)\,,\quad\caH_{222233}=\caH_{111133}\quad(15)\,,\nonumber\\
&\caH_{333322}=\caH_{333311}\quad(15)\,,\quad\caH_{333312}=-\caH_{333321}\quad(15)\,,\\
&\caH_{222333}=-\caH_{333222}\quad(10),,\quad\caH_{222331}=-\caH_{111332}\quad(60)\,,\nonumber\\
&\caH_{221133}=\caH_{112233}\quad(45)\,;\nonumber
\end{eqnarray}
however, the number of non-zero and independent component obtained into \cite{FIFU53} refers to a tensor with no major symmetries, whereas in our case $\caH=\caH^{T}$ and hence there are only 108 independent components into (\ref{4H6nonzero}). We find useful to give a tabular form for $\caH$, since it can be represented as a block matrix in terms of 6 $9\times9$ submatrices:
\begin{equation}
 % give some more room
\left[\begin{array}{@{}c|c@{}|c@{}}
\caH_{11}  & \caH_{12}\, &\caH_{13} \\ \hline
\caH_{12}^{T} & \caH_{22}\,  &\caH_{23} \\ \hline
\caH_{13}^{T} & \caH_{23}^{T}\,  &\caH_{33}
\end{array}\right]\,.
\end{equation}
with $\caH_{11}=\caH_{11}^{T}$, $\caH_{22}=\caH_{22}^{T}$ and  $\caH_{33}=\caH_{33}^{T}$. 

The tabular forms of the $9\times 9$ blocks are:
\begin{equation}
[\caH_{11}]\equiv
\left[
\begin{array}{ccccccccc}
111111   & 111122  & 111133 & 111123 & 111131  & 111112 & 111132 & 111113 & 111121\\
\cdot  & 122122  & 122133 & 122123 & 122131  & 122112 & 122132 & 122113 & 122121\\
\cdot  & \cdot  & 133133 & 133123 & 133131  & 133112 & 133132 & 133113 & 133121\\
\cdot  & \cdot  & \cdot & 123123 & 123131  & 123112 & 123132 & 123113 & 123121\\
\cdot  & \cdot  & \cdot & \cdot & 131131  & 113112 & 131132 & 131113 & 131121\\
\cdot  & \cdot  & \cdot & \cdot & \cdot  & 112112 & 112132 & 112113 & 111221\\
\cdot  & \cdot  & \cdot & \cdot & \cdot  & \cdot & 132132 & 132113 & 132121\\
\cdot  & \cdot  & \cdot & \cdot & \cdot  & \cdot & \cdot & 113113 & 113121\\
\cdot  & \cdot  & \cdot & \cdot & \cdot  & \cdot & \cdot & \cdot & 121121\\
\end{array}
\right]\,;
\end{equation}
\begin{equation}
[\caH_{22}]\equiv
\left[
\begin{array}{ccccccccc}
211211   & 211222  & 211233 & 121223 & 211231  & 211212 & 211232 & 211213 & 211221\\
\cdot  & 222222  & 222233 & 222223 & 222231  & 222212 & 222232 & 222213 & 222221\\
\cdot  & \cdot  & 233233 & 233223 & 233231  & 233212 & 233232 & 233213 & 233221\\
\cdot  & \cdot  & \cdot & 223223 & 223231  & 223212 & 223232 & 223213 & 223221\\
\cdot  & \cdot  & \cdot & \cdot & 231231  & 213212 & 231232 & 231213 & 231221\\
\cdot  & \cdot  & \cdot & \cdot & \cdot  & 212212 & 212232 & 212213 & 212221\\
\cdot  & \cdot  & \cdot & \cdot & \cdot  & \cdot & 232232 & 232213 & 232221\\
\cdot  & \cdot  & \cdot & \cdot & \cdot  & \cdot & \cdot & 213213 & 213221\\
\cdot  & \cdot  & \cdot & \cdot & \cdot  & \cdot & \cdot & \cdot & 221221\\
\end{array}
\right]\,;
\end{equation}
\begin{equation}
[\caH_{33}]\equiv
\left[
\begin{array}{ccccccccc}
311311   & 311322  & 311333 & 321323 & 311331  & 311312 & 311332 & 311313 & 311321\\
\cdot  & 322322  & 322333 & 322323 & 322331  & 322312 & 322332 & 322313 & 322321\\
\cdot  & \cdot  & 333333 & 333323 & 333331  & 333312 & 333332 & 333313 & 333321\\
\cdot  & \cdot  & \cdot & 323323 & 323331  & 323312 & 323332 & 323313 & 323321\\
\cdot  & \cdot  & \cdot & \cdot & 331331  & 313312 & 331332 & 331313 & 331321\\
\cdot  & \cdot  & \cdot & \cdot & \cdot  & 312312 & 312332 & 312313 & 312321\\
\cdot  & \cdot  & \cdot & \cdot & \cdot  & \cdot & 332332 & 332313 & 332321\\
\cdot  & \cdot  & \cdot & \cdot & \cdot  & \cdot & \cdot & 313313 & 313321\\
\cdot  & \cdot  & \cdot & \cdot & \cdot  & \cdot & \cdot & \cdot & 321321\\
\end{array}
\right]\,;
\end{equation}

\begin{equation}
[\caH_{12}]\equiv
\left[
\begin{array}{ccccccccc}
111211  & 111222  & 111233  & 111223  & 111231  & 111212  & 111213  & 111232  & 111221\\
122211  & 122222 & 122233 & 122223  & 122231  & 122212 & 122213 & 122232 & 122221 \\
133211  & 133222 & 133233 & 133223  & 133231  & 133212 & 133213 & 133232 & 133221 \\
123211  & 123222 & 123233 & 123223  & 123231  & 123212 & 123213 & 123232 & 123221\\
131211  & 131222 & 131233 & 131223  & 131231  & 131212 & 131213 & 131232 & 131221\\
112211  & 112222 & 112233 & 112223  & 112231  & 112212 & 112213 & 112232 & 112221 \\
132211  & 132222 & 132233 & 132223  & 132231  & 132212 & 132213 & 132232 & 132221 \\
113211  & 113222 & 113233 & 113223  & 113231  & 113212 & 113213 & 113232 & 113221\\
121211  & 121222 & 121233 & 121223  & 121231  & 121212 & 121213 & 121232 & 121221\\
\end{array}
\right]\,;
\end{equation}
\begin{equation}
[\caH_{13}]\equiv
\left[
\begin{array}{ccccccccc}
111311  & 111322  & 111333  & 111323  & 111331  & 111312  & 111332  & 111313  & 111321\\
122311  & 122322 & 122333 & 122323 & 122331  & 122312 & 122332 & 122313 & 122321 \\
133311  & 133322 & 133333 & 133323 & 133331  & 133312 & 133332 & 133313 & 133321 \\
123311  & 123322 & 123333 & 123323 & 123331  & 123312 & 123332 & 123313 & 123321\\
131311  & 131322 & 131333 & 131323 & 131331  & 131312 & 131332 & 131313 & 131321\\
112311  & 112322 & 112333 & 112323 & 112331  & 112312 & 112332 & 112313 & 112321 \\
132311  & 132322 & 132333 & 132323 & 132331  & 132312 & 132332 & 132313 & 132321 \\
113311  & 113322 & 113333 & 113323 & 113331  & 113312 & 113332 & 113313 & 113321\\
121311  & 121322 & 121333 & 121323 & 121331  & 121312 & 121332 & 121313 & 121321\\
\end{array}
\right]\,;
\end{equation}
\begin{equation}
[\caH_{23}]\equiv
\left[
\begin{array}{ccccccccc}
211311  & 211322  & 211333  & 211323  & 211331  & 211312  & 211332  & 211313  & 211321\\
222311  & 222322 & 222333 & 222323 & 222331  & 222312 & 222332 & 222313 & 222321 \\
233311  & 233322 & 233333 & 233323 & 233331  & 233312 & 233332 & 233313 & 233321 \\
223311  & 223322 & 223333 & 223323 & 223331  & 223312 & 223332 & 223313 & 223321\\
231311  & 231322 & 231333 & 231323 & 231331  & 231312 & 231332 & 231313 & 231321\\
212311  & 212322 & 212333 & 212323 & 212331  & 212312 & 212332 & 212313 & 212321 \\
232311  & 232322 & 232333 & 232323 & 232331  & 232312 & 232332 & 232313 & 232321 \\
213311  & 213322 & 213333 & 213323 & 213331  & 213312 & 213332 & 213313 & 213321\\
221311  & 221322 & 221333 & 221323 & 221331  & 221312 & 221332 & 221313 & 221321\\
\end{array}
\right]\,.
\end{equation}

\subsection{The acoustic tensors}

\subsubsection{The tensor $\Ab(\mb)$}

From relation (\ref{componentsHO})$_{1}$ we have the components of the second-order acoustic tensor $\Ab(\mb)$ for the classes  $4\,,\bar{4}$ and $4/m$ of the Tetragonal group, where $\bar{A}_{ij}$ 
denote the components of the acoustic tensor (\ref{Btensor}):
\begin{eqnarray}\label{acoustic1LS}
A_{11}&=&\bar{A}_{11}+\rho^{-1}(2\Del_{1111}m_{1}^{2}+2\Del_{1212}m_{2}^{2}+(\Del_{3131}+\Del_{2323})m_{3}^{2}\nonumber\\
&+&(\Del_{1112}+2\Del_{1211}-\Del_{2212})m_{1}m_{2}+\Bel_{1111}m_{1}^{2}+\Bel_{1221}m_{2}^{2}+\Bel_{2332}m_{3}^{2}\nonumber\\
&+&(\Bel_{1211}-\Bel_{2212})m_{1}m_{2})\,,\nonumber\\
A_{22}&=&\bar{A}_{22}+\rho^{-1}(2\Del_{1212}m_{1}^{2}+2\Del_{1111}m_{2}^{2}+(\Del_{3131}+\Del_{2323})m_{3}^{2}\nonumber\\
&+&(+\Del_{2212}-2\Del_{1211}-\Del_{1112})m_{1}m_{2}+\Bel_{1221}m_{1}^{2}+\Bel_{1111}m_{2}^{2}+\Bel_{2332}m_{3}^{2}\nonumber\\
&+&(\Bel_{2212}-\Bel_{1112})m_{1}m_{2})\,,\nonumber\\
A_{33}&=&\bar{A}_{33}+\rho^{-1}((\Del_{2323}+\Del_{3131}+\Bel_{2332})(m_{1}^{2}+m_{2}^{2})+(2\Del_{3333}+\Bel_{3333})m_{3}^{2})\\
A_{23}&=&\bar{A}_{23}+\rho^{-1}((\Del_{2331}-\Del_{3123})m_{1}m_{3}+(2\Del_{1133}+\Del_{2323}+\Del_{3131})m_{2}m_{3}\nonumber\\
&-&\Bel_{1233}m_{1}m_{3}+(\Bel_{1133}+\Bel_{2323})m_{2}m_{3})\,,\nonumber\\
A_{13}&=&\bar{A}_{13}+\rho^{-1}((2\Del_{1133}+\Del_{2323}+\Del_{3131})m_{1}m_{3}+(\Del_{3123}-\Del_{2331})m_{2}m_{3}\nonumber\\
&+&(\Bel_{1133}+\Bel_{3131})m_{1}m_{3}+\Bel_{1233}m_{2}m_{3})\,,\nonumber\\
A_{12}&=&\bar{A}_{12}+\rho^{-1}((\Del_{1112}-\Del_{2212})m_{1}^{2}-2\Del_{1211}m_{2}^{2}+(\Del_{3123}-\Del_{2331})m_{3}^{2}\nonumber\\
&+&2(\Del_{1122}+\Del_{1212})m_{1}m_{2}+\Bel_{1112}m_{1}^{2}+\Bel_{1222}m_{2}^{2}-\Bel_{2331}m_{3}^{2}\nonumber\\
&+&(\Bel_{1122}+\Bel_{1212})m_{1}m_{2})\,.\nonumber
\end{eqnarray}

For the higher-symmetric classes $4mmm\,,422\,,4/mm$ and $\bar{4}2m$ relations (\ref{acoustic1LS}) simplify into:
\begin{eqnarray}\label{acoustic1HS}
A_{11}&=&\bar{A}_{11}+\rho^{-1}(2\Del_{1111}m_{1}^{2}+2\Del_{1212}m_{2}^{2}+(\Del_{3131}+\Del_{2323})m_{3}^{2}\nonumber\\
&+&\Bel_{1111}m_{1}^{2}+\Bel_{1221}m_{2}^{2}+\Bel_{2332}m_{3}^{2})\nonumber\\
A_{22}&=&\bar{A}_{22}+\rho^{-1}(2\Del_{1212}m_{1}^{2}+2\Del_{1111}m_{2}^{2}+(\Del_{3131}+\Del_{2323})m_{3}^{2}\nonumber\\
&+&\Bel_{1221}m_{1}^{2}+\Bel_{1111}m_{2}^{2}+\Bel_{2332}m_{3}^{2})\\
A_{33}&=&\bar{A}_{33}+\rho^{-1}((\Del_{2323}+\Del_{3131}+\Bel_{2332})(m_{1}^{2}+m_{2}^{2})+(2\Del_{3333}+\Bel_{3333})m_{3}^{2})\nonumber\\
A_{23}&=&\bar{A}_{23}+\rho^{-1}((2\Del_{1133}+\Del_{2323}+\Del_{3131})m_{2}m_{3}+(\Bel_{1133}+\Bel_{2323})m_{2}m_{3})\,,\nonumber\\
A_{13}&=&\bar{A}_{13}+\rho^{-1}((2\Del_{1133}+\Del_{2323}+\Del_{3131})m_{1}m_{3}+(\Bel_{1133}+\Bel_{3131})m_{1}m_{3})\,,\nonumber\\
A_{12}&=&\bar{A}_{12}+\rho^{-1}(2\Del_{1122}+2\Del_{1212}+\Bel_{1122}+\Bel_{1212})m_{1}m_{2}\,.\nonumber
\end{eqnarray}

\subsubsection{The tensor $\Ael(\mb)$}

The right-hand side must be divided by the density $\rho$.
\begin{eqnarray}
\Ael_{1111}&=&\caH_{111111}m^{2}_{1}+\caH_{112112}m_{2}^{2}+\caH_{113113}m_{3}^{2}+2\caH_{111112}m_{1}m_{2}+2\caH_{111113}m_{1}m_{3}+2\caH_{112113}m_{2}m_{3}\,,\nonumber\\
\Ael_{2222}&=&\caH_{221221}m_{1}^{2}+\caH_{222222}m_{2}^{2}+\caH_{223223}m_{3}^{2}+2\caH_{221222}m_{1}m_{2}+2\caH_{221223}m_{1}m_{3}+2\caH_{222223}m_{2}m_{3}\,,\nonumber\\
\Ael_{3333}&=&\caH_{331331}m_{1}^{2}+\caH_{332332}m_{2}^{2}+\caH_{333333}m_{3}^{2}+2\caH_{331332}m_{1}m_{2}+2\caH_{331333}m_{1}m_{3}+2\caH_{332333}m_{2}m_{3}\,,\nonumber\\
\Ael_{2323}&=&\caH_{231231}m_{1}^{2}+\caH_{232232}m_{2}^{2}+\caH_{233233}m_{3}^{2}+2\caH_{231232}m_{1}m_{2}+2\caH_{231233}m_{1}m_{3}+2\caH_{232233}m_{2}m_{3}\,,\nonumber\\
\Ael_{3131}&=&\caH_{311311}m_{1}^{2}+\caH_{312312}m_{2}^{2}+\caH_{313313}m_{3}^{2}+2\caH_{311312}m_{1}m_{2}+2\caH_{311313}m_{1}m_{3}+2\caH_{312313}m_{2}m_{3}\,,\nonumber\\
\Ael_{1212}&=&\caH_{121121}m_{1}^{2}+\caH_{122122}m_{2}^{2}+\caH_{123123}m_{3}^{2}+2\caH_{121122}m_{1}m_{2}+2\caH_{121123}m_{1}m_{3}+2\caH_{122123}m_{2}m_{3}\,,\nonumber\\
\Ael_{3232}&=&\caH_{321321}m_{1}^{2}+\caH_{322322}m_{2}^{2}+\caH_{323323}m_{3}^{2}+2\caH_{321322}m_{1}m_{2}+2\caH_{321323}m_{1}m_{3}+2\caH_{322323}m_{2}m_{3}\,,\nonumber\\
\Ael_{1313}&=&\caH_{131131}m_{1}^{2}+\caH_{132132}m_{2}^{2}+\caH_{133133}m_{3}^{2}+2\caH_{131132}m_{1}m_{2}+2\caH_{131133}m_{1}m_{3}+2\caH_{132133}m_{2}m_{3}\,,\nonumber\\
\Ael_{2121}&=&\caH_{211211}m_{1}^{2}+\caH_{212212}m_{2}^{2}+\caH_{213213}m_{3}^{2}+2\caH_{211212}m_{1}m_{2}+2\caH_{211213}m_{1}m_{3}+2\caH_{212213}m_{2}m_{3}\,,\nonumber\\
\Ael_{1122}&=&\caH_{111221}m_{1}^{2}+\caH_{112222}m_{2}^{2}+\caH_{113223}m_{3}^{2}+2\caH_{111222}m_{1}m_{2}+2\caH_{111223}m_{1}m_{3}+2\caH_{112223}m_{2}m_{3}\,,\nonumber\\
\Ael_{1133}&=&\caH_{111331}m_{1}^{2}+\caH_{112332}m_{2}^{2}+\caH_{113333}m_{3}^{2}+2\caH_{111332}m_{1}m_{2}+2\caH_{111333}m_{1}m_{3}+2\caH_{112333}m_{2}m_{3}\,,\nonumber\\
\Ael_{1123}&=&\caH_{111231}m_{1}^{2}+\caH_{112232}m_{2}^{2}+\caH_{113233}m_{3}^{2}+2\caH_{111232}m_{1}m_{2}+2\caH_{111233}m_{1}m_{3}+2\caH_{112233}m_{2}m_{3}\,,\nonumber\\
\Ael_{1131}&=&\caH_{111311}m_{1}^{2}+\caH_{112312}m_{2}^{2}+\caH_{113313}m_{3}^{2}+2\caH_{111312}m_{1}m_{2}+2\caH_{111313}m_{1}m_{3}+2\caH_{112313}m_{2}m_{3}\,,\nonumber\\
\Ael_{1112}&=&\caH_{111121}m_{1}^{2}+\caH_{112122}m_{2}^{2}+\caH_{113123}m_{3}^{2}+2\caH_{111122}m_{1}m_{2}+2\caH_{111123}m_{1}m_{3}+2\caH_{112123}m_{2}m_{3}\,,\nonumber\\
\Ael_{1132}&=&\caH_{111321}m_{1}^{2}+\caH_{112322}m_{2}^{2}+\caH_{113323}m_{3}^{2}+2\caH_{111322}m_{1}m_{2}+2\caH_{111323}m_{1}m_{3}+2\caH_{112323}m_{2}m_{3}\,,\nonumber\\
\Ael_{1113}&=&\caH_{111131}m_{1}^{2}+\caH_{112132}m_{2}^{2}+\caH_{113133}m_{3}^{2}+2\caH_{111132}m_{1}m_{2}+2\caH_{111133}m_{1}m_{3}+2\caH_{112133}m_{2}m_{3}\,,\nonumber\\
\Ael_{1121}&=&\caH_{111211}m_{1}^{2}+\caH_{112212}m_{2}^{2}+\caH_{113213}m_{3}^{2}+2\caH_{111212}m_{1}m_{2}+2\caH_{111213}m_{1}m_{3}+2\caH_{112213}m_{2}m_{3}\,,\nonumber\\
\Ael_{2233}&=&\caH_{221331}m_{1}^{2}+\caH_{222332}m_{2}^{2}+\caH_{223333}m_{3}^{2}+2\caH_{221332}m_{1}m_{2}+2\caH_{221333}m_{1}m_{3}+2\caH_{222333}m_{2}m_{3}\,,\nonumber\\
\Ael_{2223}&=&\caH_{221231}m_{1}^{2}+\caH_{222232}m_{2}^{2}+\caH_{223233}m_{3}^{2}+2\caH_{221232}m_{1}m_{2}+2\caH_{221233}m_{1}m_{3}+2\caH_{222233}m_{2}m_{3}\,,\nonumber\\
\Ael_{2231}&=&\caH_{221311}m_{1}^{2}+\caH_{222312}m_{2}^{2}+\caH_{223313}m_{3}^{2}+2\caH_{221312}m_{1}m_{2}+2\caH_{221313}m_{1}m_{3}+2\caH_{222313}m_{2}m_{3}\,,\nonumber\\
\Ael_{2212}&=&\caH_{221121}m_{1}^{2}+\caH_{222122}m_{2}^{2}+\caH_{223123}m_{3}^{2}+2\caH_{221122}m_{1}m_{2}+2\caH_{221123}m_{1}m_{3}+2\caH_{222123}m_{2}m_{3}\,,\nonumber\\
\Ael_{2232}&=&\caH_{221321}m_{1}^{2}+\caH_{222322}m_{2}^{2}+\caH_{223323}m_{3}^{2}+2\caH_{221322}m_{1}m_{2}+2\caH_{221323}m_{1}m_{3}+2\caH_{222323}m_{2}m_{3}\,,\nonumber\\
\Ael_{2213}&=&\caH_{221131}m_{1}^{2}+\caH_{222132}m_{2}^{2}+\caH_{223133}m_{3}^{2}+2\caH_{221132}m_{1}m_{2}+2\caH_{221133}m_{1}m_{3}+2\caH_{222133}m_{2}m_{3}\,,\\
\Ael_{2221}&=&\caH_{221211}m_{1}^{2}+\caH_{222212}m_{2}^{2}+\caH_{223213}m_{3}^{2}+2\caH_{221212}m_{1}m_{2}+2\caH_{221213}m_{1}m_{3}+2\caH_{222213}m_{2}m_{3}\,,\nonumber\\
\Ael_{3323}&=&\caH_{331231}m_{1}^{2}+\caH_{332232}m_{2}^{2}+\caH_{333233}m_{3}^{2}+2\caH_{331232}m_{1}m_{2}+2\caH_{331233}m_{1}m_{3}+2\caH_{332233}m_{2}m_{3}\,,\nonumber\\
\Ael_{3331}&=&\caH_{331311}m_{1}^{2}+\caH_{332312}m_{2}^{2}+\caH_{333313}m_{3}^{2}+2\caH_{331312}m_{1}m_{2}+2\caH_{331313}m_{1}m_{3}+2\caH_{332313}m_{2}m_{3}\,,\nonumber\\
\Ael_{3312}&=&\caH_{331121}m_{1}^{2}+\caH_{332122}m_{2}^{2}+\caH_{333123}m_{3}^{2}+2\caH_{331122}m_{1}m_{2}+2\caH_{331123}m_{1}m_{3}+2\caH_{332123}m_{2}m_{3}\,,\nonumber\\
\Ael_{3332}&=&\caH_{331321}m_{1}^{2}+\caH_{332322}m_{2}^{2}+\caH_{333323}m_{3}^{2}+2\caH_{331322}m_{1}m_{2}+2\caH_{331323}m_{1}m_{3}+2\caH_{332323}m_{2}m_{3}\,,\nonumber\\
\Ael_{3313}&=&\caH_{331131}m_{1}^{2}+\caH_{332132}m_{2}^{2}+\caH_{333133}m_{3}^{2}+2\caH_{331132}m_{1}m_{2}+2\caH_{331133}m_{1}m_{3}+2\caH_{332133}m_{2}m_{3}\,,\nonumber
\end{eqnarray}
\begin{eqnarray}
\Ael_{3321}&=&\caH_{331211}m_{1}^{2}+\caH_{332212}m_{2}^{2}+\caH_{333213}m_{3}^{2}+2\caH_{331212}m_{1}m_{2}+2\caH_{331213}m_{1}m_{3}+2\caH_{332213}m_{2}m_{3}\,,\nonumber\\
\Ael_{2331}&=&\caH_{231311}m_{1}^{2}+\caH_{232312}m_{2}^{2}+\caH_{233313}m_{3}^{2}+2\caH_{231312}m_{1}m_{2}+2\caH_{231313}m_{1}m_{3}+2\caH_{232313}m_{2}m_{3}\,,\nonumber\\
\Ael_{2312}&=&\caH_{231121}m_{1}^{2}+\caH_{232122}m_{2}^{2}+\caH_{233123}m_{3}^{2}+2\caH_{231122}m_{1}m_{2}+2\caH_{231123}m_{1}m_{3}+2\caH_{232123}m_{2}m_{3}\,,\nonumber\\
\Ael_{2332}&=&\caH_{231321}m_{1}^{2}+\caH_{232322}m_{2}^{2}+\caH_{233323}m_{3}^{2}+2\caH_{231322}m_{1}m_{2}+2\caH_{231323}m_{1}m_{3}+2\caH_{232323}m_{2}m_{3}\,,\nonumber\\
\Ael_{2313}&=&\caH_{231131}m_{1}^{2}+\caH_{232132}m_{2}^{2}+\caH_{233133}m_{3}^{2}+2\caH_{231132}m_{1}m_{2}+2\caH_{231133}m_{1}m_{3}+2\caH_{232133}m_{2}m_{3}\,,\nonumber\\
\Ael_{2321}&=&\caH_{231211}m_{1}^{2}+\caH_{232212}m_{2}^{2}+\caH_{233213}m_{3}^{2}+2\caH_{231212}m_{1}m_{2}+2\caH_{231213}m_{1}m_{3}+2\caH_{232213}m_{2}m_{3}\,,\nonumber\\
\Ael_{3112}&=&\caH_{311131}m_{1}^{2}+\caH_{312132}m_{2}^{2}+\caH_{313133}m_{3}^{2}+2\caH_{311132}m_{1}m_{2}+2\caH_{311133}m_{1}m_{3}+2\caH_{312133}m_{2}m_{3}\,,\nonumber\\
\Ael_{3132}&=&\caH_{311321}m_{1}^{2}+\caH_{312322}m_{2}^{2}+\caH_{313323}m_{3}^{2}+2\caH_{311322}m_{1}m_{2}+2\caH_{311323}m_{1}m_{3}+2\caH_{312323}m_{2}m_{3}\,,\nonumber\\
\Ael_{3113}&=&\caH_{311131}m_{1}^{2}+\caH_{312132}m_{2}^{2}+\caH_{313133}m_{3}^{2}+2\caH_{311132}m_{1}m_{2}+2\caH_{311133}m_{1}m_{3}+2\caH_{312133}m_{2}m_{3}\,,\nonumber\\
\Ael_{3121}&=&\caH_{311211}m_{1}^{2}+\caH_{312212}m_{2}^{2}+\caH_{313213}m_{3}^{2}+2\caH_{311212}m_{1}m_{2}+2\caH_{311213}m_{1}m_{3}+2\caH_{312213}m_{2}m_{3}\,,\nonumber\\
\Ael_{1232}&=&\caH_{121321}m_{1}^{2}+\caH_{122322}m_{2}^{2}+\caH_{123323}m_{3}^{2}+2\caH_{121322}m_{1}m_{2}+2\caH_{121323}m_{1}m_{3}+2\caH_{122323}m_{2}m_{3}\,,\nonumber\\
\Ael_{1213}&=&\caH_{121131}m_{1}^{2}+\caH_{122132}m_{2}^{2}+\caH_{123133}m_{3}^{2}+2\caH_{121132}m_{1}m_{2}+2\caH_{121133}m_{1}m_{3}+2\caH_{122133}m_{2}m_{3}\,,\nonumber\\
\Ael_{1221}&=&\caH_{121211}m_{1}^{2}+\caH_{122212}m_{2}^{2}+\caH_{123213}m_{3}^{2}+2\caH_{121212}m_{1}m_{2}+2\caH_{121213}m_{1}m_{3}+2\caH_{122213}m_{2}m_{3}\,,\nonumber\\
\Ael_{3213}&=&\caH_{311131}m_{1}^{2}+\caH_{312132}m_{2}^{2}+\caH_{313133}m_{3}^{2}+2\caH_{311132}m_{1}m_{2}+2\caH_{311133}m_{1}m_{3}+2\caH_{312133}m_{2}m_{3}\,,\nonumber\\
\Ael_{3121}&=&\caH_{311211}m_{1}^{2}+\caH_{312212}m_{2}^{2}+\caH_{313213}m_{3}^{2}+2\caH_{311212}m_{1}m_{2}+2\caH_{311213}m_{1}m_{3}+2\caH_{312213}m_{2}m_{3}\,,\nonumber\\
\Ael_{1321}&=&\caH_{131211}m_{1}^{2}+\caH_{132212}m_{2}^{2}+\caH_{133213}m_{3}^{2}+2\caH_{131212}m_{1}m_{2}+2\caH_{131213}m_{1}m_{3}+2\caH_{132213}m_{2}m_{3}\,,\nonumber
\end{eqnarray}

\subsubsection{The tensor $\Pbm(\mb)$}

The right-hand side must be divided by the density $\rho$. The last two index maps tensors.
\begin{eqnarray}
\Pbm_{111}&=&(\caF_{11111}+\caG_{11111})m_{1}^{2}+(\caF_{12112}+\caG_{12112})m_{2}^{2}+(\caF_{13113}+\caG_{13113})m_{3}^{2}\nonumber\\
&+&(\caF_{11112}+\caG_{11112}+\caF_{12111}+\caG_{12111})m_{1}m_{2}\nonumber\\
&+&(\caF_{11113}+\caG_{11113}+\caF_{13111}+\caG_{13111})m_{1}m_{3}\nonumber\\
&+&(\caF_{12113}+\caG_{12113}+\caF_{13112}+\caG_{13112})m_{2}m_{3}\,,\nonumber\\
\Pbm_{122}&=&(\caF_{11221}+\caG_{11221})m_{1}^{2}+(\caF_{12222}+\caG_{12222})m_{2}^{2}+(\caF_{13223}+\caG_{13223})m_{3}^{2}\nonumber\\
&+&(\caF_{11222}+\caG_{11222}+\caF_{12221}+\caG_{12221})m_{1}m_{2}\nonumber\\
&+&(\caF_{11223}+\caG_{11223}+\caF_{13221}+\caG_{13221})m_{1}m_{3}\nonumber\\
&+&(\caF_{12223}+\caG_{12223}+\caF_{13222}+\caG_{13222})m_{2}m_{3}\,,\nonumber\\
\Pbm_{133}&=&(\caF_{11331}+\caG_{11331})m_{1}^{2}+(\caF_{12332}+\caG_{1j33p})m_{2}^{2}+(\caF_{13333}+\caG_{13333})m_{3}^{2}\nonumber\\
&+&(\caF_{11332}+\caG_{11332}+\caF_{12331}+\caG_{12331})m_{1}m_{2}\nonumber\\
&+&(\caF_{11333}+\caG_{11333}+\caF_{13331}+\caG_{13331})m_{1}m_{3}\nonumber\\
&+&(\caF_{12333}+\caG_{12333}+\caF_{13332}+\caG_{13332})m_{2}m_{3}\nonumber\,,\\
\Pbm_{123}&=&(\caF_{11231}+\caG_{11231})m_{1}^{2}+(\caF_{12232}+\caG_{12232})m_{2}^{2}+(\caF_{13233}+\caG_{13233})m_{3}^{2}\nonumber\\
&+&(\caF_{11232}+\caG_{11232}+\caF_{12231}+\caG_{12231})m_{1}m_{2}\nonumber\\
&+&(\caF_{11233}+\caG_{11233}+\caF_{13231}+\caG_{13231})m_{1}m_{3}\nonumber\\
&+&(\caF_{12233}+\caG_{12233}+\caF_{13232}+\caG_{13232})m_{2}m_{3}\,,\nonumber\\
\Pbm_{131}&=&(\caF_{11311}+\caG_{11311})m_{1}^{2}+(\caF_{12312}+\caG_{12312})m_{2}^{2}+(\caF_{13313}+\caG_{13313})m_{3}^{2}\nonumber\\
&=&(\caF_{11312}+\caG_{11312}+\caF_{12311}+\caG_{12311})m_{1}m_{2}\nonumber\\
&=&(\caF_{11313}+\caG_{11313}+\caF_{13311}+\caG_{13311})m_{1}m_{3}\nonumber\\
&=&(\caF_{12313}+\caG_{12313}+\caF_{13312}+\caG_{13312})m_{2}m_{3}\,,\nonumber\\
\Pbm_{112}&=&(\caF_{11121}+\caG_{11121})m_{1}^{2}+(\caF_{12122}+\caG_{12122})m_{2}^{2}+(\caF_{13123}+\caG_{13123})m_{3}^{2}\nonumber\\
&=&(\caF_{11122}+\caG_{11121}+\caF_{12121}+\caG_{12121})m_{1}m_{2}\nonumber\\
&=&(\caF_{11123}+\caG_{11123}+\caF_{13121}+\caG_{13121})m_{1}m_{3}\nonumber\\
&=&(\caF_{12123}+\caG_{12123}+\caF_{13122}+\caG_{13122})m_{2}m_{3}\,,\nonumber\\
\Pbm_{132}&=&(\caF_{11321}+\caG_{11321})m_{1}^{2}+(\caF_{12322}+\caG_{12322})m_{2}^{2}+(\caF_{13323}+\caG_{13323})m_{3}^{2}\nonumber\\
&=&(\caF_{11322}+\caG_{11322}+\caF_{12321}+\caG_{12321})m_{1}m_{2}\nonumber\\
&=&(\caF_{11323}+\caG_{11323}+\caF_{13321}+\caG_{13321})m_{1}m_{3}\nonumber\\
&=&(\caF_{12323}+\caG_{12323}+\caF_{13322}+\caG_{13322})m_{2}m_{3}\,,\nonumber
\end{eqnarray}
\begin{eqnarray}
\Pbm_{113}&=&(\caF_{11131}+\caG_{11131})m_{1}^{2}+(\caF_{12132}+\caG_{12132})m_{2}^{2}+(\caF_{13133}+\caG_{13133})m_{3}^{2}\nonumber\\
&=&(\caF_{11132}+\caG_{11132}+\caF_{12131}+\caG_{12131})m_{1}m_{2}\nonumber\\
&=&(\caF_{11133}+\caG_{11133}+\caF_{13131}+\caG_{13131})m_{1}m_{3}\nonumber\\
&=&(\caF_{12133}+\caG_{12133}+\caF_{13132}+\caG_{13132})m_{2}m_{3}\,,\nonumber\\
\Pbm_{121}&=&(\caF_{11211}+\caG_{11211})m_{1}^{2}+(\caF_{12212}+\caG_{12212})m_{2}^{2}+(\caF_{13213}+\caG_{13213})m_{3}^{2}\nonumber\\
&=&(\caF_{11212}+\caG_{11212}+\caF_{12211}+\caG_{12211})m_{1}m_{2}\nonumber\\
&=&(\caF_{11213}+\caG_{11213}+\caF_{13211}+\caG_{13211})m_{1}m_{3}\nonumber\\
&=&(\caF_{12213}+\caG_{12213}+\caF_{13212}+\caG_{13212})m_{2}m_{3}\nonumber\,,\\
\Pbm_{211}&=&(\caF_{21111}+\caG_{21111})m_{1}^{2}+(\caF_{22112}+\caG_{22112})m_{2}^{2}+(\caF_{23113}+\caG_{23113})m_{3}^{2}\nonumber\\
&=&(\caF_{21112}+\caG_{21112}+\caF_{22111}+\caG_{22111})m_{1}m_{2}\nonumber\\
&=&(\caF_{21113}+\caG_{21113}+\caF_{23111}+\caG_{23111})m_{1}m_{3}\nonumber\\
&=&(\caF_{22113}+\caG_{22113}+\caF_{23112}+\caG_{23112})m_{2}m_{3}\,,\nonumber\\
\Pbm_{222}&=&(\caF_{21221}+\caG_{21221})m_{1}^{2}+(\caF_{22222}+\caG_{22222})m_{2}^{2}+(\caF_{23223}+\caG_{23223})m_{3}^{2}\nonumber\\
&=&(\caF_{21222}+\caG_{21222}+\caF_{22221}+\caG_{22221})m_{1}m_{2}\nonumber\\
&=&(\caF_{21223}+\caG_{21223}+\caF_{23221}+\caG_{23221})m_{1}m_{3}\nonumber\\
&=&(\caF_{22223}+\caG_{22223}+\caF_{23221}+\caG_{23222})m_{2}m_{3}\,,\nonumber\\
\Pbm_{233}&=&(\caF_{21331}+\caG_{21331})m_{1}^{2}+(\caF_{22332}+\caG_{22332})m_{2}^{2}+(\caF_{23333}+\caG_{23333})m_{3}^{2}\nonumber\\
&=&(\caF_{21332}+\caG_{21332}+\caF_{22331}+\caG_{22331})m_{1}m_{2}\nonumber\\
&=&(\caF_{21333}+\caG_{21333}+\caF_{23331}+\caG_{23331})m_{1}m_{3}\nonumber\\
&=&(\caF_{22333}+\caG_{22333}+\caF_{23332}+\caG_{23332})m_{2}m_{3}\,,\nonumber\\
\Pbm_{223}&=&(\caF_{21331}+\caG_{21331})m_{1}^{2}+(\caF_{22332}+\caG_{22332})m_{2}^{2}+(\caF_{23333}+\caG_{23333})m_{3}^{2}\nonumber\\
&=&(\caF_{21332}+\caG_{21332}+\caF_{22331}+\caG_{22331})m_{1}m_{2}\nonumber\\
&=&(\caF_{21333}+\caG_{21333}+\caF_{23331}+\caG_{23331})m_{1}m_{3}\nonumber\\
&=&(\caF_{22333}+\caG_{22333}+\caF_{23332}+\caG_{23332})m_{2}m_{3}\,,\nonumber\\
\Pbm_{231}&=&(\caF_{21311}+\caG_{21311})m_{1}^{2}+(\caF_{22312}+\caG_{22312})m_{2}^{2}+(\caF_{23313}+\caG_{23313})m_{3}^{2}\nonumber\\
&=&(\caF_{21312}+\caG_{21312}+\caF_{22311}+\caG_{22311})m_{1}m_{2}\nonumber\\
&=&(\caF_{21313}+\caG_{21313}+\caF_{23311}+\caG_{23311})m_{1}m_{3}\nonumber\\
&=&(\caF_{22313}+\caG_{22313}+\caF_{23312}+\caG_{23312})m_{2}m_{3}\nonumber\,,\\
\Pbm_{212}&=&(\caF_{21121}+\caG_{21121})m_{1}^{2}+(\caF_{22122}+\caG_{22122})m_{2}^{2}+(\caF_{23123}+\caG_{23123})m_{3}^{2}\nonumber\\
&=&(\caF_{21122}+\caG_{21122}+(\caF_{22121}+\caG_{22121})m_{1}m_{2}\nonumber\\
&=&(\caF_{21123}+\caG_{21123}+(\caF_{23121}+\caG_{23121})m_{1}m_{3}\nonumber\\
&=&(\caF_{22123}+\caG_{22123}+(\caF_{23122}+\caG_{23122})m_{2}m_{3}\nonumber\,,
\end{eqnarray}
\begin{eqnarray}
\Pbm_{232}&=&(\caF_{21321}+\caG_{21321})m_{1}^{2}+(\caF_{22322}+\caG_{22322})m_{2}^{2}+(\caF_{23323}+\caG_{23323})m_{3}^{2}\nonumber\\
&=&(\caF_{21322}+\caG_{21322}+\caF_{22321}+\caG_{22321})m_{1}m_{2}\nonumber\\
&=&(\caF_{21323}+\caG_{21323}+\caF_{23321}+\caG_{23321})m_{1}m_{3}\nonumber\\
&=&(\caF_{22323}+\caG_{22323}+\caF_{23322}+\caG_{23322})m_{2}m_{3}\nonumber\,,\\
\Pbm_{213}&=&(\caF_{21131}+\caG_{21131})m_{1}^{2}+(\caF_{22132}+\caG_{22132})m_{2}^{2}+(\caF_{23133}+\caG_{23133})m_{3}^{2}\nonumber\\
&=&(\caF_{21132}+\caG_{21132}+\caF_{22131}+\caG_{22131})m_{1}m_{2}\nonumber\\
&=&(\caF_{21133}+\caG_{21133}+\caF_{23131}+\caG_{23131})m_{1}m_{3}\nonumber\\
&=&(\caF_{22133}+\caG_{22133}+\caF_{23132}+\caG_{23132})m_{2}m_{3}\,,\nonumber\\
\Pbm_{221}&=&(\caF_{21211}+\caG_{21211})m_{1}^{2}+(\caF_{22212}+\caG_{22212})m_{2}^{2}+(\caF_{23213}+\caG_{23213})m_{3}^{2}\nonumber\\
&=&(\caF_{21212}+\caG_{21212}+\caF_{22211}+\caG_{22211})m_{1}m_{2}\nonumber\\
&=&(\caF_{21213}+\caG_{21213}+\caF_{23211}+\caG_{23211})m_{1}m_{3}\nonumber\\
&=&(\caF_{22213}+\caG_{22213}+\caF_{23212}+\caG_{23212})m_{2}m_{3}\,,\nonumber\\
\Pbm_{311}&=&(\caF_{31111}+\caG_{31111})m_{1}^{2}+(\caF_{32112}+\caG_{32112})m_{2}^{2}+(\caF_{33113}+\caG_{33113})m_{3}^{2}\nonumber\\
&=&(\caF_{31112}+\caG_{31112}+\caF_{32111}+\caG_{32111})m_{1}m_{2}\nonumber\\
&=&(\caF_{31113}+\caG_{31113}+\caF_{33111}+\caG_{33111})m_{1}m_{3}\nonumber\\
&=&(\caF_{32113}+\caG_{32113}+\caF_{33112}+\caG_{33112})m_{2}m_{3}\,,\nonumber\\
\Pbm_{322}&=&(\caF_{31221}+\caG_{31221})m_{1}^{2}+(\caF_{32222}+\caG_{32222})m_{2}^{2}+(\caF_{33223}+\caG_{33223})m_{3}^{2}\nonumber\\
&=&(\caF_{31222}+\caG_{31222}+\caF_{32221}+\caG_{32221})m_{1}m_{2}\nonumber\\
&=&(\caF_{31223}+\caG_{31223}+\caF_{33221}+\caG_{33221})m_{1}m_{3}\nonumber\\
&=&(\caF_{32223}+\caG_{32223}+\caF_{33222}+\caG_{33222})m_{2}m_{3},,\nonumber\\
\Pbm_{333}&=&(\caF_{31331}+\caG_{31331})m_{1}^{2}+(\caF_{32332}+\caG_{32332})m_{2}^{2}+(\caF_{33333}+\caG_{33333})m_{3}^{2}\nonumber\\
&=&(\caF_{31332}+\caG_{31332}+\caF_{32331}+\caG_{32331})m_{1}m_{2}\nonumber\\
&=&(\caF_{31333}+\caG_{31333}+\caF_{33331}+\caG_{33331})m_{1}m_{3}\nonumber\\
&=&(\caF_{32333}+\caG_{32333}+\caF_{33332}+\caG_{33332})m_{2}m_{3}\,,\nonumber\\
\Pbm_{323}&=&(\caF_{31231}+\caG_{31231})m_{1}^{2}+(\caF_{32232}+\caG_{32232})m_{2}^{2}+(\caF_{33233}+\caG_{33233})m_{3}^{2}\nonumber\\
&=&(\caF_{31232}+\caG_{31232}+\caF_{32231}+\caG_{32231})m_{1}m_{2}\nonumber\\
&=&(\caF_{31233}+\caG_{31233}+\caF_{33231}+\caG_{33231})m_{1}m_{3}\nonumber\\
&=&(\caF_{32233}+\caG_{32233}+\caF_{33232}+\caG_{33232})m_{2}m_{3}\,,\nonumber\\
\Pbm_{331}&=&(\caF_{31311}+\caG_{31311})m_{1}^{2}+(\caF_{32312}+\caG_{32312})m_{2}^{2}+(\caF_{33313}+\caG_{33313})m_{3}^{2}\nonumber\\
&=&(\caF_{31312}+\caG_{31312}+\caF_{32311}+\caG_{32311})m_{1}m_{2}\nonumber\\
&=&(\caF_{31313}+\caG_{31313}+\caF_{33311}+\caG_{33311})m_{1}m_{3}\nonumber\\
&=&(\caF_{32313}+\caG_{32313}+\caF_{33312}+\caG_{33312})m_{2}m_{3}\,,\nonumber
\end{eqnarray}
\begin{eqnarray}
\Pbm_{312}&=&(\caF_{31121}+\caG_{31121})m_{1}^{2}+(\caF_{32122}+\caG_{32122})m_{2}^{2}+(\caF_{33123}+\caG_{33123})m_{3}^{2}\nonumber\\
&=&(\caF_{31122}+\caG_{31122}+\caF_{32121}+\caG_{32121})m_{1}m_{2}\nonumber\\
&=&(\caF_{31123}+\caG_{31123}+\caF_{33121}+\caG_{33121})m_{1}m_{3}\nonumber\\
&=&(\caF_{32123}+\caG_{32123}+\caF_{33121}+\caG_{33122})m_{2}m_{3}\,,\nonumber\\
\Pbm_{332}&=&(\caF_{31321}+\caG_{31321})m_{1}^{2}+(\caF_{32322}+\caG_{32322})m_{2}^{2}+(\caF_{33323}+\caG_{33323})m_{3}^{2}\nonumber\\
&=&(\caF_{31322}+\caG_{31322}+\caF_{32321}+\caG_{32321})m_{1}m_{2}\nonumber\\
&=&(\caF_{31323}+\caG_{31323}+\caF_{33321}+\caG_{33321})m_{1}m_{3}\nonumber\\
&=&(\caF_{32323}+\caG_{32323}+(\caF_{33322}+\caG_{33322})m_{2}m_{3}\,,\nonumber\\
\Pbm_{313}&=&(\caF_{31131}+\caG_{31131})m_{1}^{2}+(\caF_{32132}+\caG_{32132})m_{2}^{2}+(\caF_{33133}+\caG_{33133})m_{3}^{2}\nonumber\\
&=&(\caF_{31132}+\caG_{31132}+\caF_{32131}+\caG_{32131})m_{1}m_{2}\nonumber\\
&=&(\caF_{31133}+\caG_{31133}+\caF_{33131}+\caG_{33131})m_{1}m_{3}\nonumber\\
&=&(\caF_{32133}+\caG_{32133}+\caF_{33132}+\caG_{33132})m_{2}m_{3}\,,\nonumber\\
\Pbm_{321}&=&(\caF_{31211}+\caG_{31211})m_{1}^{2}+(\caF_{32212}+\caG_{32212})m_{2}^{2}+(\caF_{33213}+\caG_{33213})m_{3}^{2}\nonumber\\
&=&(\caF_{31212}+\caG_{31212}+\caF_{32211}+\caG_{32211})m_{1}m_{2}\nonumber\\
&=&(\caF_{31213}+\caG_{31213}+\caF_{33211}+\caG_{33211})m_{1}m_{3}\nonumber\\
&=&(\caF_{32213}+\caG_{32213}+\caF_{33212}+\caG_{33212})m_{2}m_{3}\,,\nonumber
\end{eqnarray}

\begin{equation}
[\Pbm]=
\left[
\begin{array}{ccccccccc}
  \Pbm_{111} &  \Pbm_{122}  &  \Pbm_{133}  & \Pbm_{123}& \Pbm_{131}& \Pbm_{112}& \Pbm_{132}& \Pbm_{113}& \Pbm_{121}\\
  \Pbm_{211} &  \Pbm_{222}  &  \Pbm_{233}  & \Pbm_{223}& \Pbm_{231}& \Pbm_{212}& \Pbm_{232}& \Pbm_{213}& \Pbm_{221}\\
  \Pbm_{311} &  \Pbm_{322}  &  \Pbm_{333}  & \Pbm_{323}& \Pbm_{331}& \Pbm_{312}& \Pbm_{332}& \Pbm_{313}& \Pbm_{321}\\
\end{array}
\right]
\end{equation}

\subsubsection{The tensor $\Qbm(\mb)$}

This third-order tensor is a linear function of $\mb$; for the tetragonal classes $4\,,\bar{4}$ and $4/m$ all its components are non-null. Notice that the right-hand side must be divided by the density $\rho$. 
\begin{eqnarray}
\Qbm_{111}&=&(\Del_{1111}+\Bel_{1111})m_{1}+(\Del_{1112}+\Bel_{1112})m_{2}\,,\nonumber\\
\Qbm_{122}&=&(\Del_{1212}+\Bel_{1221})m_{1}+(-\Del_{2111}+\Bel_{1222})m_{2}\,,\nonumber\\
\Qbm_{133}&=&(\Del_{3131}+\Bel_{2332})m_{1}-(\Del_{2331}+\Bel_{2331})m_{2}\,,\nonumber\\
\Qbm_{123}&=&\Bel_{1233}m_{3}\,,\nonumber\\
\Qbm_{131}&=&(\Del_{2323}+\Bel_{3131})m_{3}\,,\nonumber\\
\Qbm_{112}&=&-(\Del_{2212}+\Bel_{2212})m_{1}+(\Del_{1122}+\Bel_{1122})m_{2}\,,\nonumber\\
\Qbm_{132}&=&\Del_{3123}m_{3}\,,\nonumber\\
\Qbm_{113}&=&(\Del_{1133}+\Bel_{1133})m_{3}\,,\nonumber\\
\Qbm_{121}&=&(\Del_{1211}+\Bel_{1211})m_{1}+(\Del_{1212}+\Bel_{1212})m_{2}\,,\nonumber\\
\Qbm_{211}&=&(\Del_{1211}-\Bel_{2212})m_{1}+(\Del_{1212}+\Bel_{2112})m_{2}\,,\nonumber\\
\Qbm_{222}&=&-(\Del_{1112}+\Bel_{1112})m_{1}+(\Del_{1111}+\Bel_{1111})m_{2}\,,\nonumber\\
\Qbm_{233}&=&(\Del_{2331}+\Bel_{2331})m_{1}+(\Del_{3131}+\Bel_{2332})m_{2}\,,\nonumber\\
\Qbm_{223}&=&(\Del_{1133}+\Bel_{1133})m_{3}\,,\nonumber\\
\Qbm_{231}&=&-\Del_{3123}m_{3}\,,\\
\Qbm_{212}&=&(\Del_{1212}+\Bel_{2121})m_{1}+(-\Del_{1211}+\Bel_{2122})m_{2}\,,\nonumber\\
\Qbm_{232}&=&(\Del_{2323}+\Bel_{2323})m_{3}\,,\nonumber\\
\Qbm_{213}&=&(\Del_{2133}+\Bel_{2133})m_{3}\,,\nonumber\\
\Qbm_{221}&=&(\Del_{1122}+\Bel_{2211})m_{1}+(\Del_{2212}+\Bel_{2212})m_{2}\,,\nonumber\\
\Qbm_{311}&=&(\Del_{2323}+\Bel_{2332})m_{3}\,,\nonumber\\
\Qbm_{322}&=&(\Del_{2323}+\Bel_{3223})m_{3}\,,\nonumber\\
\Qbm_{333}&=&(\Del_{3333}+\Bel_{3333})m_{3}\,,\nonumber\\
\Qbm_{323}&=&\Del_{2331}m_{1}+(\Del_{3131}+\Bel_{2323})m_{2}\,,\nonumber\\
\Qbm_{331}&=&(\Del_{3311}+\Bel_{3311})m_{1}+(\Del_{3312}+\Bel_{3312})m_{2}\,,\nonumber\\
\Qbm_{312}&=&(\Del_{3123}+\Bel_{3123})m_{3}\,,\nonumber\\
\Qbm_{332}&=&-(\Del_{3312}+\Bel_{3312})m_{1}+(\Del_{3311}+\Bel_{3311})m_{2}\,,\nonumber\\
\Qbm_{313}&=&(\Del_{3131}+\Bel_{3131})m_{1}-\Del_{2331}m_{2}\,,\nonumber\\
\Qbm_{321}&=&-(\Del_{3123}+\Bel_{2331})m_{3}\,;\nonumber
\end{eqnarray}
we remark that 13 components depend only on $m_{3}$ and the other 14 solely on $m_{1}\,,m_{2}$.

\begin{equation}
[\Qbm]=
\left[
\begin{array}{ccccccccc}
  \Qbm_{111} &  \Qbm_{122}  &  \Qbm_{133}  & \Qbm_{123}& \Qbm_{131}& \Qbm_{112}& \Qbm_{132}& \Qbm_{113}& \Qbm_{121}\\
  \Qbm_{211} &  \Qbm_{222}  &  \Qbm_{233}  & \Qbm_{223}& \Qbm_{231}& \Qbm_{212}& \Qbm_{232}& \Qbm_{213}& \Qbm_{221}\\
  \Qbm_{311} &  \Qbm_{322}  &  \Qbm_{333}  & \Qbm_{323}& \Qbm_{331}& \Qbm_{312}& \Qbm_{332}& \Qbm_{313}& \Qbm_{321}\\
\end{array}
\right]
\end{equation}

For the other tetragonal classes we have that 6 components are zero, whereas for waves propagating along either $\eb_{1}\,,\eb_{2}$ or $\eb_{3}$ only 7 components doesn't vanish:
\begin{eqnarray}
\Qbm_{111}&=&(\Del_{1111}+\Bel_{1111})m_{1}\,,\nonumber\\
\Qbm_{122}&=&(\Del_{1212}+\Bel_{1221})m_{1}\,,\nonumber\\
\Qbm_{133}&=&(\Del_{3131}+\Bel_{2332})m_{1}\,,\nonumber\\
\Qbm_{123}&=&0\,,\nonumber\\
\Qbm_{131}&=&(\Del_{2323}+\Bel_{3131})m_{3}\,,\nonumber\\
\Qbm_{112}&=&(\Del_{1122}+\Bel_{1122})m_{2}\,,\nonumber\\
\Qbm_{132}&=&0\,,\nonumber\\
\Qbm_{113}&=&(\Del_{1133}+\Bel_{1133})m_{3}\,,\nonumber\\
\Qbm_{121}&=&(\Del_{1212}+\Bel_{1212})m_{2}\,,\nonumber\\
\Qbm_{211}&=&(\Del_{1212}+\Bel_{2112})m_{2}\,,\nonumber\\
\Qbm_{222}&=&(\Del_{1111}+\Bel_{1111})m_{2}\,,\nonumber\\
\Qbm_{233}&=&(\Del_{3131}+\Bel_{2332})m_{2}\,,\nonumber\\
\Qbm_{223}&=&(\Del_{1133}+\Bel_{1133})m_{3}\,,\nonumber\\
\Qbm_{231}&=&0\,,\\
\Qbm_{212}&=&(\Del_{1212}+\Bel_{2121})m_{1}\,,\nonumber\\
\Qbm_{232}&=&(\Del_{2323}+\Bel_{2323})m_{3}\,,\nonumber\\
\Qbm_{213}&=&0\,,\nonumber\\
\Qbm_{221}&=&(\Del_{1122}+\Bel_{2211})m_{1}\,,\nonumber\\
\Qbm_{311}&=&(\Del_{2323}+\Bel_{2332})m_{3}\,,\nonumber\\
\Qbm_{322}&=&(\Del_{2323}+\Bel_{3223})m_{3}\,,\nonumber\\
\Qbm_{333}&=&(\Del_{3333}+\Bel_{3333})m_{3}\,,\nonumber\\
\Qbm_{323}&=&(\Del_{3131}+\Bel_{2323})m_{2}\,,\nonumber\\
\Qbm_{331}&=&(\Del_{3311}+\Bel_{3311})m_{1}\,,\nonumber\\
\Qbm_{312}&=&0\,,\nonumber\\
\Qbm_{332}&=&(\Del_{3311}+\Bel_{3311})m_{2}\,,\nonumber\\
\Qbm_{313}&=&(\Del_{3131}+\Bel_{3131})m_{1}\,,\nonumber\\
\Qbm_{321}&=&0\,.\nonumber
\end{eqnarray}
